# Supplementary material for: Six-loop $\varepsilon$ expansion study of three-dimensional $n$-vector model with cubic anisotropy
Source: arXiv:1901.02754 ancillary file (2019-01-31)
Supplement: Supplementary file 1 [file rg_expansion_coefficients.pdf]

# Six-loop $\varepsilon$ expansion study of three-dimensional $n$-vector model with cubic anisotropy: supplementary materials

L. Ts. Adzhemyan[a], E. V. Ivanova[a], M. V. Kompaniets[a], A. Kudlis[a,*], A. I. Sokolov[a]

[a]*St. Petersburg State University, 7/9 Universitetskaya nab., St. Petersburg, 199034 Russia*

**Abstract**

This document contains Tables with coefficients of the six-loop RG and $\varepsilon$ expansions for three-dimensional $n$-vector model with cubic anisotropy.

## 1. Tables

Table 1: Coefficients of RG expansion for $\beta_1$

| Coef. | | Value |
|---|---|---|
| $C^{1,0}_{\beta_1}$ | | |
| | $n^0$ | $\frac{8}{3}$ |
| | $n^1$ | $\frac{1}{3}$ |
| $C^{2,0}_{\beta_1}$ | | |
| | $n^0$ | $-\frac{14}{3}$ |
| | $n^1$ | $-1$ |
| $C^{3,0}_{\beta_1}$ | | |
| | $n^0$ | $\frac{88\zeta(3)}{9}+\frac{370}{27}$ |
| | $n^1$ | $\frac{20\zeta(3)}{9}+\frac{461}{108}$ |
| | $n^2$ | $\frac{11}{72}$ |
| $C^{4,0}_{\beta_1}$ | | |
| | $n^0$ | $-\frac{4664\zeta(3)}{81}-\frac{2480\zeta(5)}{27}-\frac{24581}{486}+\frac{176\pi^4}{1215}$ |
| | $n^1$ | $-\frac{1528\zeta(3)}{81}-\frac{2200\zeta(5)}{81}-\frac{10057}{486}+\frac{62\pi^4}{1215}$ |
| | $n^2$ | $-\frac{14\zeta(3)}{9}-\frac{80\zeta(5)}{81}-\frac{395}{243}+\frac{\pi^4}{243}$ |
| | $n^3$ | $\frac{5}{3888}$ |
| Continued on next page | | |

*Corresponding author

*Email address:* `andrewkudlis@gmail.com` (A. Kudlis)

Table 1 Coefficients of RG expansion for $\beta_1$

| **Coef.** | | **Value** |
|---|---|---|
| $C_{\beta_1}^{5,0}$ | | |
| | $n^0$ | $\frac{27382\zeta(3)}{81}+\frac{1088\zeta(3)^2}{27}+\frac{55028\zeta(5)}{81}+\frac{25774\zeta(7)}{27}+\frac{17158}{81}-\frac{88\pi^4}{81}-\frac{1240\pi^6}{5103}$ |
| | $n^1$ | $\frac{69035\zeta(3)}{486}+\frac{446\zeta(3)^2}{81}+\frac{66986\zeta(5)}{243}+\frac{1029\zeta(7)}{3}+\frac{103849}{972}-\frac{2383\pi^4}{4860}-\frac{1565\pi^6}{15309}$ |
| | $n^2$ | $\frac{8455\zeta(3)}{486}-\frac{59\zeta(3)^2}{81}+\frac{7466\zeta(5)}{243}+\frac{686\zeta(7)}{27}+\frac{50531}{3888}-\frac{347\pi^4}{4860}-\frac{355\pi^6}{30618}$ |
| | $n^3$ | $\frac{26\zeta(3)}{81}-\frac{2\zeta(3)^2}{27}+\frac{305\zeta(5)}{243}+\frac{6289}{31104}-\frac{7\pi^4}{2160}-\frac{5\pi^6}{15309}$ |
| | $n^4$ | $\frac{13}{62208}-\frac{\zeta(3)}{432}$ |
| $C_{\beta_1}^{6,0}$ | | |
| | $n^0$ | $-\frac{959744\zeta(3,5)}{675}+\frac{8704\pi^4\zeta(3)}{6075}-\frac{7366714\zeta(3)}{3645}+\frac{7087432\pi^8}{9568125}+\frac{166564\pi^6}{76545}+\frac{14437\pi^4}{2025}-\frac{3117059}{3240}$ $-\frac{490552\zeta(3)^2}{405}-\frac{384512\zeta(3)^3}{729}-\frac{2940908\zeta(5)}{729}-\frac{276736\zeta(3)\zeta(5)}{81}-\frac{3306904\zeta(7)}{405}-\frac{68824768\zeta(9)}{6561}$ |
| | $n^1$ | $-\frac{44576\zeta(3,5)}{75}+\frac{6832\pi^4\zeta(3)}{18225}-\frac{762715\zeta(3)}{729}+\frac{457411\pi^8}{1366875}+\frac{790396\pi^6}{688905}+\frac{424631\pi^4}{109350}-\frac{6710257}{11664}$ $-\frac{1725208\zeta(3)^2}{3645}-\frac{158464\zeta(3)^3}{729}-\frac{2442926\zeta(5)}{1215}-\frac{97600\zeta(3)\zeta(5)}{81}-\frac{14313152\zeta(7)}{3645}-\frac{28833632\zeta(9)}{6561}$ |
| | $n^2$ | $-\frac{41968\zeta(3,5)}{675}-\frac{26\pi^4\zeta(3)}{18225}-\frac{1260521\zeta(3)}{7290}+\frac{820483\pi^8}{19136250}+\frac{6617\pi^6}{32805}+\frac{8024\pi^4}{10935}-\frac{345386}{3645}$ $-\frac{62242\zeta(3)^2}{1215}-\frac{16640\zeta(3)^3}{729}-\frac{375151\zeta(5)}{1215}-\frac{20320\zeta(3)\zeta(5)}{243}-\frac{145444\zeta(7)}{243}-\frac{3130336\zeta(9)}{6561}$ |
| | $n^3$ | $-\frac{224\zeta(3,5)}{225}-\frac{107\pi^4\zeta(3)}{18225}-\frac{23887\zeta(3)}{2916}+\frac{2063\pi^8}{1366875}+\frac{161\pi^6}{10935}+\frac{22241\pi^4}{437400}-\frac{806473}{233280}$ $+\frac{88\zeta(3)^2}{1215}-\frac{256\zeta(3)^3}{729}-\frac{131827\zeta(5)}{7290}+\frac{256\zeta(3)\zeta(5)}{243}-\frac{25339\zeta(7)}{729}-\frac{58208\zeta(9)}{6561}$ |
| | $n^4$ | $\frac{11\zeta(3)}{216}-\frac{2\pi^4\zeta(3)}{6075}+\frac{376\zeta(3)^2}{3645}-\frac{29\zeta(5)}{45}+\frac{629}{25920}+\frac{49\pi^4}{72900}+\frac{17\pi^6}{39366}$ $-\frac{88\zeta(7)}{729}$ |
| | $n^5$ | $\frac{11\zeta(3)}{19440}+\frac{29}{933120}-\frac{\pi^4}{194400}$ |
| $C_{\beta_1}^{0,1}$ | | |
| | $n^0$ | $2$ |
| $C_{\beta_1}^{1,1}$ | | |
| | $n^0$ | $-\frac{22}{3}$ |
| $C_{\beta_1}^{2,1}$ | | |
| | $n^0$ | $\frac{64\zeta(3)}{3}+\frac{659}{18}$ |
| | $n^1$ | $\frac{79}{36}$ |
| $C_{\beta_1}^{3,1}$ | | |
| | $n^0$ | $-\frac{4856\zeta(3)}{27}-\frac{2560\zeta(5)}{9}-\frac{15967}{81}+\frac{34\pi^4}{81}$ |
| | $n^1$ | $-\frac{184\zeta(3)}{9}-\frac{400\zeta(5)}{27}-\frac{1319}{54}+\frac{19\pi^4}{405}$ |
| | $n^2$ | $\frac{7}{81}-\frac{\zeta(3)}{9}$ |
| $C_{\beta_1}^{4,1}$ | | |
| | $n^0$ | $\frac{116759\zeta(3)}{81}+\frac{3148\zeta(3)^2}{27}+\frac{75236\zeta(5)}{27}+\frac{11564\zeta(7)}{3}+\frac{537437}{486}-\frac{10177\pi^4}{2430}-\frac{4810\pi^6}{5103}$ |
| | $n^1$ | $\frac{21560\zeta(3)}{81}-\frac{190\zeta(3)^2}{27}+\frac{4046\zeta(5)}{9}+\frac{1274\zeta(7)}{3}+\frac{5723}{27}-\frac{2339\pi^4}{2430}-\frac{815\pi^6}{5103}$ |
| | $n^2$ | $\frac{170\zeta(3)}{27}-\frac{4\zeta(3)^2}{3}+\frac{602\zeta(5)}{27}+\frac{59675}{15552}-\frac{19\pi^4}{360}-\frac{10\pi^6}{1701}$ |
| Continued on next page | | |

Table 1 Coefficients of RG expansion for $\beta_1$

| Coef. | | Value |
|---|---|---|
| | $n^3$ | $-\frac{17\zeta(3)}{648}+\frac{161}{10368}-\frac{\pi^4}{3240}$ |
| $C^{5,1}_{\beta_1}$ | | |
| | $n^0$ | $-\frac{1568816\zeta(3,5)}{225}+\frac{29848\pi^4\zeta(3)}{6075}-\frac{13705936\zeta(3)}{1215}+\frac{7688357\pi^8}{2126250}+\frac{817018\pi^6}{76545}+\frac{216232\pi^4}{6075}-\frac{61822279}{9720}$<br>$-\frac{2421844\zeta(3)^2}{405}-\frac{636544\zeta(3)^3}{243}-\frac{1698490\zeta(5)}{81}-\frac{1272608\zeta(3)\zeta(5)}{81}-\frac{16642943\zeta(7)}{405}-\frac{114820784\zeta(9)}{2187}$ |
| | $n^1$ | $-\frac{250744\zeta(3,5)}{225}+\frac{604\pi^4\zeta(3)}{2025}-\frac{390242\zeta(3)}{135}+\frac{9022603\pi^8}{12757500}+\frac{97348\pi^6}{32805}+\frac{13444\pi^4}{1215}-\frac{16208887}{9720}$<br>$-\frac{1210168\zeta(3)^2}{1215}-\frac{33856\zeta(3)^3}{81}-\frac{677648\zeta(5)}{135}-\frac{137312\zeta(3)\zeta(5)}{81}-\frac{2301524\zeta(7)}{243}-\frac{6313016\zeta(9)}{729}$ |
| | $n^2$ | $-\frac{1448\zeta(3,5)}{75}-\frac{568\pi^4\zeta(3)}{6075}-\frac{203771\zeta(3)}{1215}+\frac{373403\pi^8}{12757500}+\frac{41509\pi^6}{153090}+\frac{1136\pi^4}{1215}-\frac{1457371}{19440}$<br>$-\frac{2471\zeta(3)^2}{405}-\frac{1792\zeta(3)^3}{243}-\frac{277237\zeta(5)}{810}+\frac{584\zeta(3)\zeta(5)}{27}-\frac{660767\zeta(7)}{972}-\frac{407456\zeta(9)}{2187}$ |
| | $n^3$ | $\frac{523\zeta(3)}{810}-\frac{14\pi^4\zeta(3)}{2025}+\frac{2512\zeta(3)^2}{1215}-\frac{10907\zeta(5)}{810}+\frac{15317}{25920}+\frac{611\pi^4}{36450}+\frac{827\pi^6}{91854}$<br>$-\frac{616\zeta(7)}{243}$ |
| | $n^4$ | $\frac{37\zeta(3)}{2430}-\frac{\zeta(5)}{108}+\frac{23}{8640}-\frac{19\pi^4}{291600}$ |
| $C^{0,2}_{\beta_1}$ | | |
| | $n^0$ | $-\frac{5}{3}$ |
| $C^{1,2}_{\beta_1}$ | | |
| | $n^0$<br>$n^1$ | $8\zeta(3)+\frac{107}{4}$<br>$\frac{1}{24}$ |
| $C^{2,2}_{\beta_1}$ | | |
| | $n^0$<br>$n^1$ | $-\frac{1456\zeta(3)}{9}-\frac{2000\zeta(5)}{9}-\frac{13433}{54}+\frac{32\pi^4}{135}$<br>$-\frac{35\zeta(3)}{9}-\frac{301}{72}$ |
| $C^{3,2}_{\beta_1}$ | | |
| | $n^0$<br>$n^1$<br>$n^2$ | $\frac{171533\zeta(3)}{81}+\frac{1384\zeta(3)^2}{27}+\frac{96794\zeta(5)}{27}+\frac{14210\zeta(7)}{3}+\frac{1314497}{648}-\frac{4621\pi^4}{972}-\frac{5080\pi^6}{5103}$<br>$\frac{9230\zeta(3)}{81}-\frac{232\zeta(3)^2}{27}+\frac{2045\zeta(5)}{9}+\frac{245\zeta(7)}{3}+\frac{270749}{2592}-\frac{4841\pi^4}{9720}-\frac{290\pi^6}{5103}$<br>$\frac{763\zeta(3)}{648}+\frac{5\zeta(5)}{9}-\frac{1921}{10368}-\frac{17\pi^4}{3240}$ |
| $C^{4,2}_{\beta_1}$ | | |
| | $n^0$ | $-\frac{834896\zeta(3,5)}{75}+\frac{2516\pi^4\zeta(3)}{1215}-\frac{5747761\zeta(3)}{243}+\frac{12101801\pi^8}{2126250}+\frac{433787\pi^6}{25515}+\frac{2265121\pi^4}{36450}-\frac{903730709}{58320}$<br>$-\frac{1434952\zeta(3)^2}{135}-\frac{39296\zeta(3)^3}{9}-\frac{3086303\zeta(5)}{81}-\frac{595504\zeta(3)\zeta(5)}{27}-\frac{56870887\zeta(7)}{810}-\frac{7181008\zeta(9)}{81}$ |
| | $n^1$ | $-\frac{11352\zeta(3,5)}{25}-\frac{1628\pi^4\zeta(3)}{6075}-\frac{975469\zeta(3)}{405}+\frac{564199\pi^8}{1417500}+\frac{232003\pi^6}{91854}+\frac{176576\pi^4}{18225}-\frac{170986643}{116640}$<br>$-\frac{125420\zeta(3)^2}{243}-192\zeta(3)^3-\frac{1962497\zeta(5)}{486}-\frac{5320\zeta(3)\zeta(5)}{27}-\frac{4100653\zeta(7)}{540}-\frac{38504\zeta(9)}{9}$ |
| | $n^2$ | $-\frac{8\zeta(3,5)}{5}-\frac{359\pi^4\zeta(3)}{6075}-\frac{15599\zeta(3)}{540}+\frac{2063\pi^8}{850500}+\frac{46429\pi^6}{459270}+\frac{27791\pi^4}{97200}-\frac{370891}{233280}$<br>$+\frac{15346\zeta(3)^2}{1215}-\frac{341159\zeta(5)}{2430}-\frac{56\zeta(3)\zeta(5)}{27}-\frac{181513\zeta(7)}{1620}$ |
| | $n^3$ | $\frac{89\zeta(3)}{19440}-\frac{\zeta(3)^2}{27}-\frac{29\zeta(5)}{60}-\frac{475}{186624}+\frac{769\pi^4}{583200}+\frac{\pi^6}{10206}$ |
| $C^{0,3}_{\beta_1}$ | | |
| | $n^0$ | 7 |
| | | Continued on next page |

Table 1 Coefficients of RG expansion for $\beta_1$

| **Coef.** | | **Value** |
|---|---|---|
| $C_{\beta_1}^{1,3}$ | | |
| | $n^0$ | $-50\zeta(3) - \frac{160\zeta(5)}{3} - \frac{4867}{36} - \frac{4\pi^4}{45}$ |
| | $n^1$ | $\frac{\zeta(3)}{3} - \frac{25}{36}$ |
| $C_{\beta_1}^{2,3}$ | | |
| | $n^0$ | $\frac{37789\zeta(3)}{27} - \frac{544\zeta(3)^2}{9} + \frac{17444\zeta(5)}{9} + 2352\zeta(7) + \frac{2281727}{1296} - \frac{337\pi^4}{270} - \frac{320\pi^6}{1701}$ |
| | $n^1$ | $\frac{344\zeta(3)}{27} + \frac{208\zeta(5)}{9} + \frac{30277}{1296} - \frac{5\pi^4}{108}$ |
| $C_{\beta_1}^{3,3}$ | | |
| | $n^0$ | $-\frac{189408\zeta(3,5)}{25} - \frac{15476\pi^4\zeta(3)}{2025} - \frac{10058446\zeta(3)}{405} + \frac{419233\pi^8}{118125} + \frac{87233\pi^6}{8505} + \frac{556567\pi^4}{12150} - \frac{73299097}{3888} - \frac{421396\zeta(3)^2}{45} - \frac{89600\zeta(3)^3}{27} - \frac{4440497\zeta(5)}{135} - \frac{100528\zeta(3)\zeta(5)}{9} - \frac{14652953\zeta(7)}{270} - \frac{16719808\zeta(9)}{243}$ |
| | $n^1$ | $-\frac{1008\zeta(3,5)}{25} - \frac{154\pi^4\zeta(3)}{2025} - \frac{7911\zeta(3)}{10} + \frac{2063\pi^8}{33750} + \frac{17129\pi^6}{21870} + \frac{140717\pi^4}{48600} - \frac{7223929}{12960} - \frac{5684\zeta(3)^2}{81} - \frac{640\zeta(3)^3}{27} - \frac{1055113\zeta(5)}{810} + \frac{904\zeta(3)\zeta(5)}{9} - \frac{234083\zeta(7)}{108} - \frac{145520\zeta(9)}{243}$ |
| | $n^2$ | $-\frac{248\zeta(3)}{405} - \frac{142\zeta(3)^2}{135} - \frac{2791\zeta(5)}{270} - \frac{112\zeta(7)}{27} - \frac{4735}{1944} + \frac{419\pi^4}{12150} + \frac{23\pi^6}{7290}$ |
| $C_{\beta_1}^{0,4}$ | | |
| | $n^0$ | $-3\zeta(3) - \frac{477}{16} - \frac{\pi^4}{15}$ |
| $C_{\beta_1}^{1,4}$ | | |
| | $n^0$ | $\frac{5495\zeta(3)}{12} - \frac{190\zeta(3)^2}{3} + \frac{1145\zeta(5)}{3} + 441\zeta(7) + \frac{1336801}{1728} + \frac{47\pi^4}{60} + \frac{115\pi^6}{567}$ |
| | $n^1$ | $-\frac{77\zeta(3)}{48} - \frac{4\zeta(5)}{3} + \frac{26171}{6912} + \frac{7\pi^4}{720}$ |
| $C_{\beta_1}^{2,4}$ | | |
| | $n^0$ | $-\frac{54496\zeta(3,5)}{25} - \frac{7447\pi^4\zeta(3)}{675} - \frac{11815331\zeta(3)}{810} + \frac{182113\pi^8}{354375} + \frac{4838\pi^6}{25515} + \frac{71243\pi^4}{6480} - \frac{65729015}{5184} - \frac{636224\zeta(3)^2}{135} - \frac{11200\zeta(3)^3}{9} - \frac{1961179\zeta(5)}{135} + 72\zeta(3)\zeta(5) - \frac{274364\zeta(7)}{15} - \frac{2141384\zeta(9)}{81}$ |
| | $n^1$ | $-\frac{606731\zeta(3)}{6480} + \frac{17\pi^4\zeta(3)}{150} - \frac{44\zeta(3)^2}{9} - \frac{3298\zeta(5)}{45} - \frac{2740145}{20736} + \frac{737\pi^4}{12960} + \frac{229\pi^6}{8505} - \frac{17441\zeta(7)}{90}$ |
| $C_{\beta_1}^{0,5}$ | | |
| | $n^0$ | $\frac{1519\zeta(3)}{24} - 18\zeta(3)^2 + 2\zeta(5) + \frac{158849}{1152} + \frac{13\pi^4}{36} + \frac{5\pi^6}{63}$ |
| $C_{\beta_1}^{1,5}$ | | |
| | $n^0$ | $-\frac{1512\zeta(3,5)}{25} - \frac{1331\pi^4\zeta(3)}{225} - \frac{1692407\zeta(3)}{360} - \frac{2579\pi^8}{7500} - \frac{36277\pi^6}{17010} - \frac{26477\pi^4}{10800} - \frac{78802267}{17280} - \frac{61417\zeta(3)^2}{45} - 192\zeta(3)^3 - \frac{270109\zeta(5)}{90} + 2056\zeta(3)\zeta(5) - \frac{36629\zeta(7)}{30} - \frac{12536\zeta(9)}{3}$ |
| | $n^1$ | $\frac{7\zeta(3)}{360} + \frac{\pi^4\zeta(3)}{50} - \frac{13\zeta(3)^2}{15} + \frac{361\zeta(5)}{20} - \frac{351589}{17280} - \frac{53\pi^4}{600} - \frac{37\pi^6}{5670} + \frac{107\zeta(7)}{15}$ |
| $C_{\beta_1}^{0,6}$ | | |
| | $n^0$ | $\frac{1944\zeta(3,5)}{25} - \frac{6\pi^4\zeta(3)}{5} - \frac{472891\zeta(3)}{720} - \frac{2063\pi^8}{17500} - \frac{163\pi^6}{270} - \frac{113\pi^4}{96} - \frac{7915913}{11520} - \frac{892\zeta(3)^2}{5} - \frac{4019\zeta(5)}{20} + 576\zeta(3)\zeta(5) + \frac{4629\zeta(7)}{10}$ |

Table 2: Coefficients of RG expansion for $\beta_2$

| **Coef.** | | **Value** |
|---|---|---|
| $C_{\beta_2}^{1,0}$ | | |
| | $n^0$ | $3$ |
| $C_{\beta_2}^{2,0}$ | | |
| | $n^0$ | $-\frac{17}{3}$ |
| $C_{\beta_2}^{3,0}$ | | |
| | $n^0$ | $12\zeta(3) + \frac{145}{8}$ |
| $C_{\beta_2}^{4,0}$ | | |
| | $n^0$ | $-78\zeta(3) - 120\zeta(5) - \frac{3499}{48} + \frac{\pi^4}{5}$ |
| $C_{\beta_2}^{5,0}$ | | |
| | $n^0$ | $\frac{7965\zeta(3)}{16} + 45\zeta(3)^2 + 987\zeta(5) + 1323\zeta(7) + \frac{764621}{2304} - \frac{1189\pi^4}{720} - \frac{5\pi^6}{14}$ |
| $C_{\beta_2}^{6,0}$ | | |
| | $n^0$ | $-\frac{51984\zeta(3,5)}{25} + \frac{9\pi^4\zeta(3)}{5} - \frac{779603\zeta(3)}{240} + \frac{88181\pi^8}{78750} + \frac{6691\pi^6}{1890} + \frac{5663\pi^4}{480} - \frac{18841427}{11520}$ $-\frac{8678\zeta(3)^2}{5} - 768\zeta(3)^3 - \frac{63723\zeta(5)}{10} - 4704\zeta(3)\zeta(5) - \frac{63627\zeta(7)}{5} - \frac{46112\zeta(9)}{3}$ |
| $C_{\beta_2}^{0,1}$ | | |
| | $n^0$ | $4$ |
| $C_{\beta_2}^{1,1}$ | | |
| | $n^0$ | $-\frac{46}{3}$ |
| $C_{\beta_2}^{2,1}$ | | |
| | $n^0$ | $48\zeta(3) + \frac{131}{2}$ |
| $C_{\beta_2}^{3,1}$ | | |
| | $n^0$ | $-387\zeta(3) - 600\zeta(5) - \frac{1004}{3} + \frac{16\pi^4}{15}$ |
| $C_{\beta_2}^{4,1}$ | | |
| | $n^0$ | $\frac{35083\zeta(3)}{12} + 288\zeta(3)^2 + 5920\zeta(5) + 7938\zeta(7) + \frac{1067507}{576} - \frac{3697\pi^4}{360} - \frac{20\pi^6}{9}$ |
| $C_{\beta_2}^{5,1}$ | | |
| | $n^0$ | $-\frac{365832\zeta(3,5)}{25} + \frac{69\pi^4\zeta(3)}{5} - \frac{3974693\zeta(3)}{180} + \frac{1253101\pi^8}{157500} + \frac{3427\pi^6}{135} + \frac{6701\pi^4}{80} - \frac{10331173}{960}$ $-\frac{59854\zeta(3)^2}{5} - 5376\zeta(3)^3 - \frac{888103\zeta(5)}{20} - 33504\zeta(3)\zeta(5) - \frac{895407\zeta(7)}{10} - \frac{322784\zeta(9)}{3}$ |
| $C_{\beta_2}^{0,2}$ | | |
| | $n^0$ | $-\frac{82}{9}$ |
| | $n^1$ | $-\frac{5}{9}$ |
| $C_{\beta_2}^{1,2}$ | | |
| | $n^0$ | $64\zeta(3) + \frac{325}{4}$ |
| | $n^1$ | $\frac{17}{24}$ |
| | | Continued on next page |

Table 2 Coefficients of RG expansion for $\beta_2$

| Coef. | | Value |
|---|---|---|
| $C_{\beta_2}^{2,2}$ | | |
| | $n^0$ | $-724\zeta(3) - \frac{3440\zeta(5)}{3} - \frac{10661}{18} + \frac{92\pi^4}{45}$ |
| | $n^1$ | $-\frac{19\zeta(3)}{3} - \frac{19}{24} + \frac{2\pi^4}{45}$ |
| $C_{\beta_2}^{3,2}$ | | |
| | $n^0$ | $\frac{125459\zeta(3)}{18} + \frac{2266\zeta(3)^2}{3} + 14328\zeta(5) + 19404\zeta(7) + \frac{3633377}{864} - \frac{2263\pi^4}{90} - \frac{445\pi^6}{81}$ |
| | $n^1$ | $\frac{2947\zeta(3)}{72} - 17\zeta(3)^2 + \frac{290\zeta(5)}{3} - \frac{16223}{3456} - \frac{151\pi^4}{360} - \frac{25\pi^6}{378}$ |
| $C_{\beta_2}^{4,2}$ | | |
| | $n^0$ | $-\frac{1088208\zeta(3,5)}{25} + \frac{9887\pi^4\zeta(3)}{225} - \frac{1139269\zeta(3)}{18} + \frac{207733\pi^8}{8750} + \frac{128659\pi^6}{1701} + \frac{99007\pi^4}{400} - \frac{51557351}{1728}$ $-\frac{1582436\zeta(3)^2}{45} - 15936\zeta(3)^3 - \frac{1951531\zeta(5)}{15} - 101128\zeta(3)\zeta(5) - \frac{3965812\zeta(7)}{15} - \frac{955816\zeta(9)}{3}$ |
| | $n^1$ | $-\frac{1944\zeta(3,5)}{25} - \frac{37\pi^4\zeta(3)}{150} - \frac{53143\zeta(3)}{240} + \frac{2063\pi^8}{17500} + \frac{4799\pi^6}{5670} + \frac{60019\pi^4}{21600} + \frac{2444831}{34560}$ $+\frac{250\zeta(3)^2}{3} - \frac{131953\zeta(5)}{180} + 288\zeta(3)\zeta(5) - \frac{16321\zeta(7)}{10}$ |
| $C_{\beta_2}^{0,3}$ | | |
| | $n^0$ | $\frac{224\zeta(3)}{9} + \frac{821}{27}$ |
| | $n^1$ | $\frac{16\zeta(3)}{9} + \frac{92}{27}$ |
| | $n^2$ | $-\frac{13}{108}$ |
| $C_{\beta_2}^{1,3}$ | | |
| | $n^0$ | $-\frac{5312\zeta(3)}{9} - 960\zeta(5) - \frac{12349}{27} + \frac{44\pi^4}{27}$ |
| | $n^1$ | $-\frac{218\zeta(3)}{9} - \frac{160\zeta(5)}{9} - \frac{508}{27} + \frac{2\pi^4}{15}$ |
| | $n^2$ | $\frac{\zeta(3)}{9} + \frac{1}{6}$ |
| $C_{\beta_2}^{2,3}$ | | |
| | $n^0$ | $\frac{224804\zeta(3)}{27} + \frac{3032\zeta(3)^2}{3} + \frac{155692\zeta(5)}{9} + 23912\zeta(7) + \frac{9309907}{1944} - \frac{36509\pi^4}{1215} - \frac{20\pi^6}{3}$ |
| | $n^1$ | $\frac{1309\zeta(3)}{6} - \frac{452\zeta(3)^2}{9} + 478\zeta(5) + 196\zeta(7) + \frac{496159}{7776} - \frac{2038\pi^4}{1215} - \frac{70\pi^6}{243}$ |
| | $n^2$ | $-\frac{35\zeta(3)}{108} + \frac{14\zeta(5)}{9} + \frac{8213}{15552} - \frac{\pi^4}{135}$ |
| $C_{\beta_2}^{3,3}$ | | |
| | $n^0$ | $-\frac{1749344\zeta(3,5)}{25} + \frac{50468\pi^4\zeta(3)}{675} - \frac{39442336\zeta(3)}{405} + \frac{13456907\pi^8}{354375} + \frac{608252\pi^6}{5103} + \frac{3133897\pi^4}{8100} - \frac{7974529}{180}$ $-\frac{7583302\zeta(3)^2}{135} - \frac{229760\zeta(3)^3}{9} - \frac{27534421\zeta(5)}{135} - \frac{1488176\zeta(3)\zeta(5)}{9} - 417463\zeta(7) - \frac{41246416\zeta(9)}{81}$ |
| | $n^1$ | $-624\zeta(3,5) - \frac{547\pi^4\zeta(3)}{675} - \frac{658271\zeta(3)}{405} + \frac{6653\pi^8}{9450} + \frac{1813\pi^6}{405} + \frac{13451\pi^4}{900} - \frac{783227}{6480}$ $+\frac{6463\zeta(3)^2}{45} - \frac{320\zeta(3)^3}{3} - \frac{240961\zeta(5)}{54} + \frac{5768\zeta(3)\zeta(5)}{9} - \frac{846977\zeta(7)}{90} - \frac{62680\zeta(9)}{27}$ |
| | $n^2$ | $\frac{11\zeta(3)}{5} - \frac{17\pi^4\zeta(3)}{450} + \frac{29\zeta(3)^2}{45} - \frac{407\zeta(5)}{45} - \frac{56759}{6480} + \frac{239\pi^4}{8100} + \frac{47\pi^6}{2430}$ $-\frac{1369\zeta(7)}{45}$ |
| $C_{\beta_2}^{0,4}$ | | |
| | $n^0$ | $-168\zeta(3) - \frac{7280\zeta(5)}{27} - \frac{19679}{162} + \frac{4\pi^4}{9}$ |
| | $n^1$ | $-\frac{560\zeta(3)}{27} - \frac{280\zeta(5)}{9} - \frac{3479}{162} + \frac{34\pi^4}{405}$ |
| | | Continued on next page |

Table 2 Coefficients of RG expansion for $\beta_2$

| **Coef.** | | **Value** |
|---|---|---|
| | $n^2$ | $-\frac{8\zeta(3)}{9}-\frac{7}{162}+\frac{2\pi^4}{405}$ |
| | $n^3$ | $\frac{\zeta(3)}{27}-\frac{29}{1296}$ |
| $C_{\beta_2}^{1,4}$ | | |
| | $n^0$ | $\frac{784621\zeta(3)}{162}+\frac{18154\zeta(3)^2}{27}+\frac{275510\zeta(5)}{27}+\frac{43120\zeta(7)}{3}+\frac{1279979}{486}-\frac{83837\pi^4}{4860}-\frac{19795\pi^6}{5103}$ |
| | $n^1$ | $\frac{31598\zeta(3)}{81}-\frac{1045\zeta(3)^2}{27}+\frac{20917\zeta(5)}{27}+\frac{1960\zeta(7)}{3}+\frac{11495}{54}-\frac{10729\pi^4}{4860}-\frac{4285\pi^6}{10206}$ |
| | $n^2$ | $\zeta(3)-\frac{4\zeta(3)^2}{3}+\frac{364\zeta(5)}{27}-\frac{43295}{31104}-\frac{121\pi^4}{2160}-\frac{10\pi^6}{1701}$ |
| | $n^3$ | $-\frac{91\zeta(3)}{1296}+\frac{127}{20736}+\frac{\pi^4}{1620}$ |
| $C_{\beta_2}^{2,4}$ | | |
| | $n^0$ | $-\frac{4746464\zeta(3,5)}{75}+\frac{144076\pi^4\zeta(3)}{2025}-\frac{101821793\zeta(3)}{1215}+\frac{36052067\pi^8}{1063125}+\frac{1589395\pi^6}{15309}+\frac{450349\pi^4}{1350}-\frac{710623019}{19440}$ <br> $-\frac{20594684\zeta(3)^2}{405}-23040\zeta(3)^3-\frac{72318487\zeta(5)}{405}-\frac{1374928\zeta(3)\zeta(5)}{9}-\frac{33092563\zeta(7)}{90}-\frac{4122304\zeta(9)}{9}$ |
| | $n^1$ | $-\frac{140176\zeta(3,5)}{75}-\frac{92\pi^4\zeta(3)}{405}-\frac{5168816\zeta(3)}{1215}+\frac{3532181\pi^8}{2126250}+\frac{453707\pi^6}{51030}+\frac{7345\pi^4}{243}-\frac{49494349}{38880}$ <br> $-\frac{65008\zeta(3)^2}{135}-\frac{4480\zeta(3)^3}{9}-\frac{8245481\zeta(5)}{810}-\frac{7400\zeta(3)\zeta(5)}{9}-\frac{2269039\zeta(7)}{108}-\frac{853328\zeta(9)}{81}$ |
| | $n^2$ | $-\frac{144\zeta(3,5)}{25}-\frac{137\pi^4\zeta(3)}{675}-\frac{30911\zeta(3)}{4860}+\frac{2063\pi^8}{236250}+\frac{776\pi^6}{5103}+\frac{4019\pi^4}{10800}-\frac{327553}{77760}$ <br> $+\frac{2999\zeta(3)^2}{135}-\frac{32684\zeta(5)}{405}+\frac{64\zeta(3)\zeta(5)}{3}-\frac{21821\zeta(7)}{90}$ |
| | $n^3$ | $-\frac{1607\zeta(3)}{6480}-\frac{\zeta(3)^2}{45}-\frac{23\zeta(5)}{45}+\frac{144449}{311040}-\frac{217\pi^4}{194400}+\frac{\pi^6}{2835}$ |
| $C_{\beta_2}^{0,5}$ | | |
| | $n^0$ | $\frac{259358\zeta(3)}{243}+\frac{13288\zeta(3)^2}{81}+\frac{179696\zeta(5)}{81}+\frac{28420\zeta(7)}{9}+\frac{389095}{729}-\frac{13583\pi^4}{3645}-\frac{12700\pi^6}{15309}$ |
| | $n^1$ | $\frac{15742\zeta(3)}{81}-\frac{92\zeta(3)^2}{81}+\frac{34460\zeta(5)}{81}+490\zeta(7)+\frac{95588}{729}-\frac{3296\pi^4}{3645}-\frac{2950\pi^6}{15309}$ |
| | $n^2$ | $\frac{2785\zeta(3)}{243}-\frac{92\zeta(3)^2}{81}+\frac{530\zeta(5)}{27}+\frac{98\zeta(7)}{9}+\frac{111217}{23328}-\frac{211\pi^4}{2916}-\frac{190\pi^6}{15309}$ |
| | $n^3$ | $-\frac{151\zeta(3)}{972}+\frac{8\zeta(5)}{81}-\frac{3557}{46656}-\frac{2\pi^4}{1215}$ |
| | $n^4$ | $-\frac{5\zeta(3)}{972}-\frac{61}{15552}+\frac{\pi^4}{9720}$ |
| $C_{\beta_2}^{1,5}$ | | |
| | $n^0$ | $-\frac{2217616\zeta(3,5)}{75}+\frac{71168\pi^4\zeta(3)}{2025}-\frac{1009990\zeta(3)}{27}+\frac{33205421\pi^8}{2126250}+\frac{712604\pi^6}{15309}+\frac{12014\pi^4}{81}-\frac{149700341}{9720}$ <br> $-\frac{9756916\zeta(3)^2}{405}-\frac{291200\zeta(3)^3}{27}-\frac{404788\zeta(5)}{5}-\frac{1977728\zeta(3)\zeta(5)}{27}-\frac{68024194\zeta(7)}{405}-\frac{51926224\zeta(9)}{243}$ |
| | $n^1$ | $-\frac{62072\zeta(3,5)}{25}+\frac{2356\pi^4\zeta(3)}{2025}-\frac{1869658\zeta(3)}{405}+\frac{2500139\pi^8}{1417500}+\frac{599374\pi^6}{76545}+\frac{105961\pi^4}{4050}-\frac{3178819}{1620}$ <br> $-\frac{101300\zeta(3)^2}{81}-\frac{21056\zeta(3)^3}{27}-\frac{464938\zeta(5)}{45}-\frac{89888\zeta(3)\zeta(5)}{27}-\frac{8347004\zeta(7)}{405}-\frac{3898552\zeta(9)}{243}$ |
| | $n^2$ | $-\frac{696\zeta(3,5)}{25}-\frac{166\pi^4\zeta(3)}{675}-\frac{16645\zeta(3)}{162}+\frac{59827\pi^8}{1417500}+\frac{5104\pi^6}{15309}+\frac{9367\pi^4}{8100}-\frac{372449}{19440}$ <br> $+\frac{10303\zeta(3)^2}{405}-\frac{128\zeta(3)^3}{27}-\frac{99019\zeta(5)}{405}+\frac{1328\zeta(3)\zeta(5)}{27}-\frac{120455\zeta(7)}{162}-\frac{29104\zeta(9)}{243}$ |
| | $n^3$ | $\frac{947\zeta(3)}{540}-\frac{4\pi^4\zeta(3)}{675}+\frac{208\zeta(3)^2}{135}-\frac{383\zeta(5)}{135}-\frac{59}{648}-\frac{4\pi^4}{1215}+\frac{113\pi^6}{25515}$ <br> $-\frac{176\zeta(7)}{81}$ |
| | $n^4$ | $-\frac{\zeta(3)}{135}+\frac{\zeta(5)}{36}-\frac{53}{25920}-\frac{7\pi^4}{32400}$ |
| $C_{\beta_2}^{0,6}$ | | |
| | $n^0$ | $-\frac{3580576\zeta(3,5)}{675}+\frac{123088\pi^4\zeta(3)}{18225}-\frac{24155126\zeta(3)}{3645}+\frac{26546953\pi^8}{9568125}+\frac{1863808\pi^6}{229635}+\frac{477067\pi^4}{18225}-\frac{72730159}{29160}$ |
| | | Continued on next page |

Table 2 Coefficients of RG expansion for $\beta_2$

| Coef. | | Value |
|---|---|---|
| | $n^1$ | $-\frac{5457904\zeta(3)^2}{1215}-\frac{472832\zeta(3)^3}{243}-\frac{10395416\zeta(5)}{729}-\frac{3266240\zeta(3)\zeta(5)}{243}-\frac{36159098\zeta(7)}{1215}-\frac{84043936\zeta(9)}{2187}$ $-\frac{737984\zeta(3,5)}{675}+\frac{4784\pi^4\zeta(3)}{6075}-\frac{5964733\zeta(3)}{3645}+\frac{6369302\pi^8}{9568125}+\frac{1718846\pi^6}{688905}+\frac{173677\pi^4}{21870}-\frac{46378889}{58320}$ |
| | $n^2$ | $-\frac{2390588\zeta(3)^2}{3645}-\frac{3328\zeta(3)^3}{9}-\frac{1514048\zeta(5)}{405}-\frac{167456\zeta(3)\zeta(5)}{81}-\frac{67279\zeta(7)}{9}-\frac{202208\zeta(9)}{27}$ $-\frac{1272\zeta(3,5)}{25}-\frac{286\pi^4\zeta(3)}{6075}-\frac{328069\zeta(3)}{2430}+\frac{190817\pi^8}{4252500}+\frac{166736\pi^6}{688905}+\frac{1804\pi^4}{2187}-\frac{837679}{14580}$ |
| | $n^3$ | $-\frac{82088\zeta(3)^2}{3645}-\frac{3776\zeta(3)^3}{243}-\frac{105292\zeta(5)}{405}-\frac{8432\zeta(3)\zeta(5)}{243}-\frac{281611\zeta(7)}{486}-\frac{719464\zeta(9)}{2187}$ $-\frac{8\zeta(3,5)}{15}-\frac{97\pi^4\zeta(3)}{18225}-\frac{9079\zeta(3)}{4860}+\frac{2063\pi^8}{2551500}+\frac{263\pi^6}{39366}+\frac{14479\pi^4}{437400}+\frac{30757}{77760}$ |
| | $n^4$ | $+\frac{4237\zeta(3)^2}{3645}-\frac{12818\zeta(5)}{3645}+\frac{40\zeta(3)\zeta(5)}{243}-\frac{14599\zeta(7)}{972}$ $\frac{3823\zeta(3)}{29160}+\frac{8\zeta(3)^2}{243}-\frac{4\zeta(5)}{243}-\frac{1123}{38880}-\frac{367\pi^4}{437400}+\frac{\pi^6}{45927}$ |
| | $n^5$ | $-\frac{13\zeta(3)}{11664}+\frac{\zeta(5)}{324}-\frac{125}{186624}-\frac{\pi^4}{69984}$ |

Table 3: Coefficients of RG expansion for $\gamma_\varphi$

| **Coef.** | | **Value** |
|---|---|---|
| $C_{\gamma_\varphi}^{2,0}$ | | |
| | $n^0$ | $\frac{1}{18}$ |
| | $n^1$ | $\frac{1}{36}$ |
| $C_{\gamma_\varphi}^{3,0}$ | | |
| | $n^0$ | $-\frac{1}{27}$ |
| | $n^1$ | $-\frac{5}{216}$ |
| | $n^2$ | $-\frac{1}{432}$ |
| $C_{\gamma_\varphi}^{4,0}$ | | |
| | $n^0$ | $\frac{125}{648}$ |
| | $n^1$ | $\frac{85}{648}$ |
| | $n^2$ | $\frac{5}{324}$ |
| | $n^3$ | $-\frac{5}{5184}$ |
| $C_{\gamma_\varphi}^{5,0}$ | | |
| | $n^0$ | $\frac{23\zeta(3)}{243} - \frac{602}{729} - \frac{11\pi^4}{3645}$ |
| | $n^1$ | $\frac{13\zeta(3)}{162} - \frac{1915}{2916} - \frac{8\pi^4}{3645}$ |
| | $n^2$ | $\frac{13\zeta(3)}{972} - \frac{1459}{11664} - \frac{\pi^4}{2916}$ |
| | $n^3$ | $-\frac{\zeta(3)}{972} - \frac{187}{93312}$ |
| | $n^4$ | $\frac{\zeta(3)}{3888} - \frac{13}{62208}$ |
| $C_{\gamma_\varphi}^{6,0}$ | | |
| | $n^0$ | $\frac{581\zeta(3)}{729} - \frac{62\zeta(3)^2}{243} - \frac{1628\zeta(5)}{729} + \frac{88159}{23328} + \frac{269\pi^4}{14580} + \frac{155\pi^6}{45927}$ |
| | $n^1$ | $\frac{427\zeta(3)}{729} - \frac{148\zeta(3)^2}{729} - \frac{925\zeta(5)}{486} + \frac{156797}{46656} + \frac{1369\pi^4}{87480} + \frac{370\pi^6}{137781}$ |
| | $n^2$ | $\frac{65\zeta(3)}{486} - \frac{59\zeta(3)^2}{1458} - \frac{37\zeta(5)}{81} + \frac{9523}{11664} + \frac{161\pi^4}{43740} + \frac{295\pi^6}{551124}$ |
| | $n^3$ | $\frac{13\zeta(3)}{648} - \frac{\zeta(3)^2}{729} - \frac{185\zeta(5)}{5832} + \frac{2383}{62208} + \frac{83\pi^4}{349920} + \frac{5\pi^6}{275562}$ |
| | $n^4$ | $-\frac{\zeta(3)}{23328} - \frac{71}{62208} + \frac{\pi^4}{349920}$ |
| | $n^5$ | $-\frac{\zeta(3)}{46656} - \frac{29}{746496} + \frac{\pi^4}{1399680}$ |
| $C_{\gamma_\varphi}^{1,1}$ | | |
| | $n^0$ | $\frac{1}{6}$ |
| $C_{\gamma_\varphi}^{2,1}$ | | |
| | $n^0$ | $-\frac{1}{6}$ |
| | $n^1$ | $-\frac{1}{48}$ |
| $C_{\gamma_\varphi}^{3,1}$ | | |
| | $n^0$ | $\frac{125}{108}$ |
| | $n^1$ | $\frac{5}{24}$ |
| | | Continued on next page |

Table 3 Coefficients of RG expansion for $\gamma_\varphi$

| **Coef.** | | **Value** |
|---|---|---|
| | $n^2$ | $-\frac{5}{432}$ |
| $C^{4,1}_{\gamma_\varphi}$ | | |
| | $n^0$ | $\frac{115\zeta(3)}{162}-\frac{1505}{243}-\frac{11\pi^4}{486}$ |
| | $n^1$ | $\frac{20\zeta(3)}{81}-\frac{395}{216}-\frac{5\pi^4}{972}$ |
| | $n^2$ | $-\frac{5\zeta(3)}{216}-\frac{185}{7776}$ |
| | $n^3$ | $\frac{5\zeta(3)}{1296}-\frac{65}{20736}$ |
| $C^{5,1}_{\gamma_\varphi}$ | | |
| | $n^0$ | $\frac{581\zeta(3)}{81}-\frac{62\zeta(3)^2}{27}-\frac{1628\zeta(5)}{81}+\frac{88159}{2592}+\frac{269\pi^4}{1620}+\frac{155\pi^6}{5103}$ |
| | $n^1$ | $\frac{91\zeta(3)}{54}-\frac{55\zeta(3)^2}{81}-\frac{1147\zeta(5)}{162}+\frac{34319}{2592}+\frac{281\pi^4}{4860}+\frac{275\pi^6}{30618}$ |
| | $n^2$ | $\frac{13\zeta(3)}{36}-\frac{2\zeta(3)^2}{81}-\frac{185\zeta(5)}{324}+\frac{3773}{5184}+\frac{41\pi^4}{9720}+\frac{5\pi^6}{15309}$ |
| | $n^3$ | $\frac{\pi^4}{38880}-\frac{397}{20736}$ |
| | $n^4$ | $-\frac{\zeta(3)}{2592}-\frac{29}{41472}+\frac{\pi^4}{77760}$ |
| $C^{0,2}_{\gamma_\varphi}$ | | |
| | $n^0$ | $\frac{1}{12}$ |
| $C^{1,2}_{\gamma_\varphi}$ | | |
| | $n^0$ | $-\frac{3}{16}$ |
| $C^{2,2}_{\gamma_\varphi}$ | | |
| | $n^0$ | $\frac{145}{72}$ |
| | $n^1$ | $\frac{5}{288}$ |
| $C^{3,2}_{\gamma_\varphi}$ | | |
| | $n^0$ | $\frac{191\zeta(3)}{108}-\frac{58177}{3888}-\frac{13\pi^4}{243}$ |
| | $n^1$ | $\frac{23\zeta(3)}{216}-\frac{4453}{3888}-\frac{\pi^4}{486}$ |
| | $n^2$ | $\frac{325}{31104}$ |
| $C^{4,2}_{\gamma_\varphi}$ | | |
| | $n^0$ | $\frac{101563\zeta(3)}{4860}-\frac{187\zeta(3)^2}{27}-\frac{6623\zeta(5)}{108}+\frac{8181029}{77760}+\frac{12301\pi^4}{24300}+\frac{935\pi^6}{10206}$ |
| | $n^1$ | $\frac{3823\zeta(3)}{1944}-\frac{31\zeta(3)^2}{54}-\frac{5143\zeta(5)}{648}+\frac{461041}{31104}+\frac{77\pi^4}{1215}+\frac{155\pi^6}{20412}$ |
| | $n^2$ | $\frac{1799\zeta(3)}{9720}-\frac{37\zeta(5)}{324}-\frac{40241}{311040}+\frac{259\pi^4}{388800}$ |
| | $n^3$ | $-\frac{13\zeta(3)}{5184}-\frac{293}{248832}+\frac{\pi^4}{17280}$ |
| $C^{0,3}_{\gamma_\varphi}$ | | |
| | $n^0$ | $-\frac{1}{16}$ |
| $C^{1,3}_{\gamma_\varphi}$ | | |
| | $n^0$ | $\frac{65}{48}$ |
| $C^{2,3}_{\gamma_\varphi}$ | | |
| | $n^0$ | $\frac{67\zeta(3)}{36}-\frac{13741}{864}-\frac{\pi^4}{18}$ |
| | | Continued on next page |

Table 3 Coefficients of RG expansion for $\gamma_\varphi$

| **Coef.** | | **Value** |
|---|---|---|
| | $n^1$ | $\frac{\zeta(3)}{72}-\frac{671}{3456}$ |
| $C_{\gamma_\varphi}^{3,3}$ | | |
| | $n^0$<br>$n^1$<br>$n^2$ | $\frac{48191\zeta(3)}{1620}-\frac{266\zeta(3)^2}{27}-\frac{2405\zeta(5)}{27}+\frac{3988303}{25920}+\frac{2971\pi^4}{4050}+\frac{95\pi^6}{729}$<br>$\frac{3161\zeta(3)}{3240}-\frac{4\zeta(3)^2}{27}-\frac{185\zeta(5)}{54}+\frac{103931}{17280}+\frac{581\pi^4}{21600}+\frac{10\pi^6}{5103}$<br>$\frac{13\zeta(3)}{2160}-\frac{1723}{103680}-\frac{\pi^4}{16200}$ |
| $C_{\gamma_\varphi}^{0,4}$ | | |
| | $n^0$ | $\frac{65}{192}$ |
| $C_{\gamma_\varphi}^{1,4}$ | | |
| | $n^0$ | $\frac{15\zeta(3)}{16}-\frac{18545}{2304}-\frac{\pi^4}{36}$ |
| $C_{\gamma_\varphi}^{2,4}$ | | |
| | $n^0$<br>$n^1$ | $\frac{24727\zeta(3)}{1080}-\frac{15\zeta(3)^2}{2}-\frac{2479\zeta(5)}{36}+\frac{1371179}{11520}+\frac{24467\pi^4}{43200}+\frac{25\pi^6}{252}$<br>$\frac{1309\zeta(3)}{8640}-\frac{37\zeta(5)}{72}+\frac{40309}{46080}+\frac{341\pi^4}{86400}$ |
| $C_{\gamma_\varphi}^{0,5}$ | | |
| | $n^0$ | $\frac{3\zeta(3)}{16}-\frac{3709}{2304}-\frac{\pi^4}{180}$ |
| $C_{\gamma_\varphi}^{1,5}$ | | |
| | $n^0$ | $\frac{295\zeta(3)}{32}-3\zeta(3)^2-\frac{111\zeta(5)}{4}+\frac{73667}{1536}+\frac{73\pi^4}{320}+\frac{5\pi^6}{126}$ |
| $C_{\gamma_\varphi}^{0,6}$ | | |
| | $n^0$ | $\frac{295\zeta(3)}{192}-\frac{\zeta(3)^2}{2}-\frac{37\zeta(5)}{8}+\frac{73667}{9216}+\frac{73\pi^4}{1920}+\frac{5\pi^6}{756}$ |

Table 4: Coefficients of RG expansion for $\gamma_{m^2}$

| Coef. | | Value |
|---|---|---|
| $C^{1,0}_{\gamma_{m^2}}$ | | |
| | $n^0$ | $-1$ |
| $C^{2,0}_{\gamma_{m^2}}$ | | |
| | $n^0$ | $\frac{5}{6}$ |
| $C^{3,0}_{\gamma_{m^2}}$ | | |
| | $n^0$ | $-\frac{7}{2}$ |
| $C^{4,0}_{\gamma_{m^2}}$ | | |
| | $n^0$ | $\frac{3\zeta(3)}{2}+\frac{477}{32}+\frac{\pi^4}{30}$ |
| $C^{5,0}_{\gamma_{m^2}}$ | | |
| | $n^0$ | $-\frac{1519\zeta(3)}{48}+9\zeta(3)^2-\zeta(5)-\frac{158849}{2304}-\frac{13\pi^4}{72}-\frac{5\pi^6}{126}$ |
| $C^{6,0}_{\gamma_{m^2}}$ | | |
| | $n^0$ | $-\frac{972\zeta(3,5)}{25}+\frac{3\pi^4\zeta(3)}{5}+\frac{472891\zeta(3)}{1440}+\frac{2063\pi^8}{35000}+\frac{163\pi^6}{540}+\frac{113\pi^4}{192}+\frac{7915913}{23040}$ $+\frac{446\zeta(3)^2}{5}+\frac{4019\zeta(5)}{40}-288\zeta(3)\zeta(5)-\frac{4629\zeta(7)}{20}$ |
| $C^{0,1}_{\gamma_{m^2}}$ | | |
| | $n^0$<br>$n^1$ | $-\frac{2}{3}$<br>$-\frac{1}{3}$ |
| $C^{1,1}_{\gamma_{m^2}}$ | | |
| | $n^0$ | $\frac{5}{3}$ |
| $C^{2,1}_{\gamma_{m^2}}$ | | |
| | $n^0$<br>$n^1$ | $-\frac{251}{24}$<br>$-\frac{1}{24}$ |
| $C^{3,1}_{\gamma_{m^2}}$ | | |
| | $n^0$<br>$n^1$ | $\frac{19\zeta(3)}{3}+\frac{4243}{72}+\frac{2\pi^4}{15}$<br>$\frac{25}{36}-\frac{\zeta(3)}{3}$ |
| $C^{4,1}_{\gamma_{m^2}}$ | | |
| | $n^0$<br>$n^1$ | $-\frac{959\zeta(3)}{6}+45\zeta(3)^2-\frac{19\zeta(5)}{3}-\frac{589141}{1728}-\frac{643\pi^4}{720}-\frac{25\pi^6}{126}$<br>$\frac{77\zeta(3)}{48}+\frac{4\zeta(5)}{3}-\frac{26171}{6912}-\frac{7\pi^4}{720}$ |
| $C^{5,1}_{\gamma_{m^2}}$ | | |
| | $n^0$<br><br>$n^1$ | $-\frac{5832\zeta(3,5)}{25}+\frac{181\pi^4\zeta(3)}{50}+\frac{1418687\zeta(3)}{720}+\frac{6189\pi^8}{17500}+\frac{5116\pi^6}{2835}+\frac{8263\pi^4}{2400}+\frac{70540039}{34560}$ $+\frac{1603\zeta(3)^2}{3}+\frac{6209\zeta(5)}{10}-1728\zeta(3)\zeta(5)-\frac{41447\zeta(7)}{30}$<br>$-\frac{7\zeta(3)}{360}-\frac{\pi^4\zeta(3)}{50}+\frac{13\zeta(3)^2}{15}-\frac{361\zeta(5)}{20}+\frac{351589}{17280}+\frac{53\pi^4}{600}+\frac{37\pi^6}{5670}$ $-\frac{107\zeta(7)}{15}$ |

Continued on next page

Table 4 Coefficients of RG expansion for $\gamma_{m^2}$

| **Coef.** | | **Value** |
|---|---|---|
| $C^{0,2}_{\gamma_{m^2}}$ | | |
| | $n^0$ | $\frac{5}{9}$ |
| | $n^1$ | $\frac{5}{18}$ |
| $C^{1,2}_{\gamma_{m^2}}$ | | |
| | $n^0$ | $-\frac{37}{4}$ |
| | $n^1$ | $-\frac{5}{4}$ |
| $C^{2,2}_{\gamma_{m^2}}$ | | |
| | $n^0$ | $\frac{26\zeta(3)}{3}+\frac{9199}{108}+\frac{26\pi^4}{135}$ |
| | $n^1$ | $\frac{\zeta(3)}{3}+\frac{1841}{432}+\frac{\pi^4}{135}$ |
| $C^{3,2}_{\gamma_{m^2}}$ | | |
| | $n^0$ | $-\frac{627\zeta(3)}{2}+\frac{806\zeta(3)^2}{9}-\frac{118\zeta(5)}{9}-\frac{32003}{48}-\frac{95\pi^4}{54}-\frac{95\pi^6}{243}$ |
| | $n^1$ | $-\frac{71\zeta(3)}{24}+\frac{4\zeta(3)^2}{9}+\frac{28\zeta(5)}{9}-\frac{26173}{1152}-\frac{5\pi^4}{108}-\frac{10\pi^6}{1701}$ |
| $C^{4,2}_{\gamma_{m^2}}$ | | |
| | $n^0$ | $-\frac{14472\zeta(3,5)}{25}+\frac{2038\pi^4\zeta(3)}{225}+\frac{1312903\zeta(3)}{270}+\frac{138221\pi^8}{157500}+\frac{12631\pi^6}{2835}+\frac{61289\pi^4}{7200}+\frac{260283349}{51840}$ <br> $+1327\zeta(3)^2+\frac{70262\zeta(5)}{45}-4300\zeta(3)\zeta(5)-\frac{41033\zeta(7)}{12}$ |
| | $n^1$ | $-\frac{108\zeta(3,5)}{25}-\frac{13\pi^4\zeta(3)}{225}+\frac{273647\zeta(3)}{4320}+\frac{2063\pi^8}{315000}+\frac{821\pi^6}{11340}+\frac{4547\pi^4}{14400}+\frac{27514859}{207360}$ <br> $+11\zeta(3)^2-\frac{19531\zeta(5)}{360}-20\zeta(3)\zeta(5)-\frac{157\zeta(7)}{3}$ |
| $C^{0,3}_{\gamma_{m^2}}$ | | |
| | $n^0$ | $-\frac{37}{18}$ |
| | $n^1$ | $-\frac{47}{36}$ |
| | $n^2$ | $-\frac{5}{36}$ |
| $C^{1,3}_{\gamma_{m^2}}$ | | |
| | $n^0$ | $\frac{136\zeta(3)}{27}+\frac{7765}{162}+\frac{44\pi^4}{405}$ |
| | $n^1$ | $\frac{20\zeta(3)}{27}+\frac{421}{36}+\frac{2\pi^4}{81}$ |
| | $n^2$ | $\frac{2\zeta(3)}{9}-\frac{1}{648}$ |
| $C^{2,3}_{\gamma_{m^2}}$ | | |
| | $n^0$ | $-\frac{47327\zeta(3)}{162}+\frac{2308\zeta(3)^2}{27}-\frac{310\zeta(5)}{27}-\frac{267737}{432}-\frac{8039\pi^4}{4860}-\frac{1870\pi^6}{5103}$ |
| | $n^1$ | $-\frac{3743\zeta(3)}{162}+\frac{122\zeta(3)^2}{27}+\frac{11\zeta(5)}{9}-\frac{362281}{5184}-\frac{1493\pi^4}{9720}-\frac{155\pi^6}{5103}$ |
| | $n^2$ | $-\frac{785\zeta(3)}{648}+\frac{7\zeta(5)}{27}+\frac{2045}{10368}+\frac{7\pi^4}{3240}$ |
| $C^{3,3}_{\gamma_{m^2}}$ | | |
| | $n^0$ | $-\frac{3744\zeta(3,5)}{5}+\frac{7984\pi^4\zeta(3)}{675}+\frac{1680331\zeta(3)}{270}+\frac{26819\pi^8}{23625}+\frac{146156\pi^6}{25515}+\frac{270437\pi^4}{24300}+\frac{250114079}{38880}$ <br> $+\frac{232714\zeta(3)^2}{135}+\frac{273689\zeta(5)}{135}-\frac{16784\zeta(3)\zeta(5)}{3}-\frac{597154\zeta(7)}{135}$ |
| | $n^1$ | $-\frac{144\zeta(3,5)}{5}+\frac{346\pi^4\zeta(3)}{2025}+\frac{553121\zeta(3)}{1620}+\frac{2063\pi^8}{47250}+\frac{7789\pi^6}{25515}+\frac{7199\pi^4}{10800}+\frac{11362699}{25920}$ <br> $+\frac{1603\zeta(3)^2}{27}-\frac{5213\zeta(5)}{270}-\frac{496\zeta(3)\zeta(5)}{3}-\frac{9134\zeta(7)}{45}$ |
| | | Continued on next page |

Table 4 Coefficients of RG expansion for $\gamma_{m^2}$

| **Coef.** | | **Value** |
|---|---|---|
| | $n^2$ | $\frac{9881\zeta(3)}{3240}+\frac{2\pi^4\zeta(3)}{2025}+\frac{37\zeta(3)^2}{45}+\frac{40\zeta(5)}{27}+\frac{3149}{31104}-\frac{1207\pi^4}{48600}+\frac{2\pi^6}{567}-\frac{359\zeta(7)}{135}$ |
| $C^{0,4}_{\gamma_{m^2}}$ | | |
| | $n^0$ | $\frac{68\zeta(3)}{81}+\frac{7765}{972}+\frac{22\pi^4}{1215}$ |
| | $n^1$ | $\frac{44\zeta(3)}{81}+\frac{5777}{972}+\frac{16\pi^4}{1215}$ |
| | $n^2$ | $\frac{8\zeta(3)}{81}+\frac{947}{972}+\frac{\pi^4}{486}$ |
| | $n^3$ | $\frac{\zeta(3)}{54}-\frac{1}{7776}$ |
| $C^{1,4}_{\gamma_{m^2}}$ | | |
| | $n^0$ | $-\frac{6635\zeta(3)}{54}+\frac{970\zeta(3)^2}{27}-\frac{40\zeta(5)}{9}-\frac{247385}{972}-\frac{667\pi^4}{972}-\frac{775\pi^6}{5103}$ |
| | $n^1$ | $-\frac{95\zeta(3)}{3}+\frac{725\zeta(3)^2}{81}-\frac{70\zeta(5)}{81}-\frac{4675}{54}-\frac{17\pi^4}{81}-\frac{1375\pi^6}{30618}$ |
| | $n^2$ | $-\frac{1175\zeta(3)}{324}+\frac{10\zeta(3)^2}{81}+\frac{25\zeta(5)}{81}-\frac{113135}{31104}-\frac{29\pi^4}{3888}-\frac{25\pi^6}{15309}$ |
| | $n^3$ | $-\frac{85\zeta(3)}{1296}-\frac{35}{20736}+\frac{\pi^4}{1296}$ |
| $C^{2,4}_{\gamma_{m^2}}$ | | |
| | $n^0$ | $-\frac{2576\zeta(3,5)}{5}+\frac{50006\pi^4\zeta(3)}{6075}+\frac{1716683\zeta(3)}{405}+\frac{47449\pi^8}{60750}+\frac{200329\pi^6}{51030}+\frac{281423\pi^4}{36450}+\frac{508665283}{116640}+\frac{32321\zeta(3)^2}{27}+\frac{1143833\zeta(5)}{810}-\frac{34936\zeta(3)\zeta(5)}{9}-\frac{4956361\zeta(7)}{1620}$ |
| | $n^1$ | $-\frac{336\zeta(3,5)}{5}+\frac{103\pi^4\zeta(3)}{135}+\frac{3206107\zeta(3)}{4860}+\frac{2063\pi^8}{20250}+\frac{177347\pi^6}{306180}+\frac{43183\pi^4}{36450}+\frac{183687439}{233280}+\frac{110411\zeta(3)^2}{810}+\frac{133819\zeta(5)}{1620}-\frac{3908\zeta(3)\zeta(5)}{9}-\frac{1283101\zeta(7)}{3240}$ |
| | $n^2$ | $-\frac{4\zeta(3,5)}{5}+\frac{34\pi^4\zeta(3)}{6075}+\frac{266333\zeta(3)}{9720}+\frac{2063\pi^8}{1701000}+\frac{6961\pi^6}{306180}-\frac{43343\pi^4}{583200}+\frac{2362241}{466560}+\frac{3757\zeta(3)^2}{810}+\frac{1999\zeta(5)}{162}-4\zeta(3)\zeta(5)-\frac{17549\zeta(7)}{1080}$ |
| | $n^3$ | $\frac{5099\zeta(3)}{38880}-\frac{\zeta(3)^2}{45}+\frac{\zeta(5)}{24}+\frac{241291}{1866240}-\frac{3581\pi^4}{1166400}+\frac{11\pi^6}{102060}$ |
| $C^{0,5}_{\gamma_{m^2}}$ | | |
| | $n^0$ | $-\frac{1327\zeta(3)}{81}+\frac{388\zeta(3)^2}{81}-\frac{16\zeta(5)}{27}-\frac{49477}{1458}-\frac{667\pi^4}{7290}-\frac{310\pi^6}{15309}$ |
| | $n^1$ | $-\frac{2011\zeta(3)}{162}+\frac{872\zeta(3)^2}{243}-\frac{100\zeta(5)}{243}-\frac{83137}{2916}-\frac{215\pi^4}{2916}-\frac{740\pi^6}{45927}$ |
| | $n^2$ | $-\frac{1261\zeta(3)}{486}+\frac{149\zeta(3)^2}{243}-\frac{4\zeta(5)}{243}-\frac{291907}{46656}-\frac{437\pi^4}{29160}-\frac{295\pi^6}{91854}$ |
| | $n^3$ | $-\frac{487\zeta(3)}{1944}+\frac{2\zeta(3)^2}{243}+\frac{5\zeta(5)}{243}-\frac{2831}{11664}-\frac{23\pi^4}{58320}-\frac{5\pi^6}{45927}$ |
| | $n^4$ | $-\frac{17\zeta(3)}{3888}-\frac{7}{62208}+\frac{\pi^4}{19440}$ |
| $C^{1,5}_{\gamma_{m^2}}$ | | |
| | $n^0$ | $-\frac{4208\zeta(3,5)}{25}+\frac{5512\pi^4\zeta(3)}{2025}+\frac{562321\zeta(3)}{405}+\frac{542569\pi^8}{2126250}+\frac{32672\pi^6}{25515}+\frac{30583\pi^4}{12150}+\frac{9092683}{6480}+\frac{53344\zeta(3)^2}{135}+\frac{37652\zeta(5)}{81}-\frac{11488\zeta(3)\zeta(5)}{9}-\frac{135677\zeta(7)}{135}$ |
| | $n^1$ | $-\frac{1512\zeta(3,5)}{25}+\frac{5024\pi^4\zeta(3)}{6075}+\frac{208918\zeta(3)}{405}+\frac{2063\pi^8}{22500}+\frac{36884\pi^6}{76545}+\frac{2429\pi^4}{2430}+\frac{1315433}{2160}+\frac{52288\zeta(3)^2}{405}+\frac{17309\zeta(5)}{135}-\frac{3824\zeta(3)\zeta(5)}{9}-\frac{56905\zeta(7)}{162}$ |
| | $n^2$ | $-\frac{112\zeta(3,5)}{25}+\frac{314\pi^4\zeta(3)}{6075}+\frac{11641\zeta(3)}{180}+\frac{2063\pi^8}{303750}+\frac{3589\pi^6}{76545}+\frac{137\pi^4}{4860}+\frac{214759}{4320}+\frac{4328\zeta(3)^2}{405}+\frac{6101\zeta(5)}{810}-\frac{80\zeta(3)\zeta(5)}{3}-\frac{2518\zeta(7)}{81}$ |
| | $n^3$ | $\frac{1151\zeta(3)}{810}-\frac{4\pi^4\zeta(3)}{6075}+\frac{4\zeta(3)^2}{15}+\frac{1811\zeta(5)}{810}-\frac{8039}{17280}-\frac{1303\pi^4}{97200}+\frac{19\pi^6}{10206}$ |
| | | Continued on next page |

Table 4 Coefficients of RG expansion for $\gamma_{m^2}$

| Coef. | | Value |
|---|---|---|
| | | $-\frac{4\zeta(7)}{3}$ |
| | $n^4$ | $-\frac{17\zeta(3)}{2160}+\frac{\zeta(5)}{36}-\frac{43}{103680}-\frac{47\pi^4}{194400}$ |
| $C^{0,6}_{\gamma_{m^2}}$ | | |
| | $n^0$ | $-\frac{4208\zeta(3,5)}{225}+\frac{5512\pi^4\zeta(3)}{18225}+\frac{562321\zeta(3)}{3645}+\frac{542569\pi^8}{19136250}+\frac{32672\pi^6}{229635}+\frac{30583\pi^4}{109350}+\frac{9092683}{58320}$ $+\frac{53344\zeta(3)^2}{1215}+\frac{37652\zeta(5)}{729}-\frac{11488\zeta(3)\zeta(5)}{81}-\frac{135677\zeta(7)}{1215}$ |
| | $n^1$ | $-\frac{3616\zeta(3,5)}{225}+\frac{13292\pi^4\zeta(3)}{54675}+\frac{326719\zeta(3)}{2430}+\frac{233119\pi^8}{9568125}+\frac{85892\pi^6}{688905}+\frac{6097\pi^4}{24300}+\frac{16985281}{116640}$ $+\frac{132304\zeta(3)^2}{3645}+\frac{146057\zeta(5)}{3645}-\frac{9568\zeta(3)\zeta(5)}{81}-\frac{345778\zeta(7)}{3645}$ |
| | $n^2$ | $-\frac{868\zeta(3,5)}{225}+\frac{314\pi^4\zeta(3)}{6075}+\frac{104521\zeta(3)}{2916}+\frac{63953\pi^8}{10935000}+\frac{22031\pi^6}{688905}+\frac{1283\pi^4}{21870}+\frac{31879}{810}$ $+\frac{30472\zeta(3)^2}{3645}+\frac{29014\zeta(5)}{3645}-\frac{2152\zeta(3)\zeta(5)}{81}-\frac{66977\zeta(7)}{2916}$ |
| | $n^3$ | $-\frac{56\zeta(3,5)}{225}+\frac{17\pi^4\zeta(3)}{6075}+\frac{109373\zeta(3)}{29160}+\frac{2063\pi^8}{5467500}+\frac{1937\pi^6}{688905}+\frac{67\pi^4}{874800}+\frac{46831}{17280}$ $+\frac{2272\zeta(3)^2}{3645}+\frac{3241\zeta(5)}{4860}-\frac{40\zeta(3)\zeta(5)}{27}-\frac{1367\zeta(7)}{729}$ |
| | $n^4$ | $\frac{4553\zeta(3)}{58320}-\frac{2\pi^4\zeta(3)}{54675}+\frac{2\zeta(3)^2}{135}+\frac{464\zeta(5)}{3645}-\frac{151}{5832}-\frac{\pi^4}{1296}+\frac{19\pi^6}{183708}$ $-\frac{2\zeta(7)}{27}$ |
| | $n^5$ | $-\frac{17\zeta(3)}{38880}+\frac{\zeta(5)}{648}-\frac{43}{1866240}-\frac{47\pi^4}{3499200}$ |

Table 5: Coefficients of $\varepsilon$ expansion for $g_1^*$

| **Coef.** | | **Value** |
|---|---|---|
| $C_{g_1}^{(3)}$ | | |
| | $n^{-1}$ | $\frac{8\zeta(3)}{9} - \frac{1955}{5832}$ |
| | $n^{-2}$ | $-\frac{8\zeta(3)}{3} - \frac{41971}{5832}$ |
| | $n^{-3}$ | $\frac{38329}{972} - \frac{28\zeta(3)}{9}$ |
| | $n^{-4}$ | $\frac{56\zeta(3)}{9} - \frac{45080}{729}$ |
| | $n^{-5}$ | $\frac{22472}{729}$ |
| $C_{g_1}^{(4)}$ | | |
| | $n^{-1}$ | $\frac{110\zeta(3)}{243} - \frac{80\zeta(5)}{27} - \frac{2987}{314928} + \frac{\pi^4}{135}$ |
| | $n^{-2}$ | $\frac{2744\zeta(3)}{243} + \frac{80\zeta(5)}{9} + \frac{113779}{104976} - \frac{8\pi^4}{405}$ |
| | $n^{-3}$ | $-\frac{7934\zeta(3)}{243} + \frac{80\zeta(5)}{27} - \frac{3955061}{52488} - \frac{8\pi^4}{405}$ |
| | $n^{-4}$ | $-\frac{12764\zeta(3)}{243} + \frac{200\zeta(5)}{27} + \frac{8315992}{19683} + \frac{16\pi^4}{405}$ |
| | $n^{-5}$ | $\frac{46696\zeta(3)}{243} - \frac{80\zeta(5)}{3} - \frac{5934115}{6561}$ |
| | $n^{-6}$ | $\frac{5623300}{6561} - \frac{29680\zeta(3)}{243}$ |
| | $n^{-7}$ | $-\frac{5955080}{19683}$ |
| $C_{g_1}^{(5)}$ | | |
| | $n^{-1}$ | $\frac{13883\zeta(3)}{34992} - \frac{16\zeta(3)^2}{27} - \frac{340\zeta(5)}{243} + \frac{98\zeta(7)}{9} - \frac{5795035}{136048896} + \frac{217\pi^4}{58320} - \frac{20\pi^6}{5103}$ |
| | $n^{-2}$ | $-\frac{182483\zeta(3)}{34992} - \frac{296\zeta(3)^2}{81} - \frac{26296\zeta(5)}{729} - \frac{343\zeta(7)}{9} + \frac{337198481}{136048896} + \frac{3929\pi^4}{43740} + \frac{170\pi^6}{15309}$ |
| | $n^{-3}$ | $\frac{653341\zeta(3)}{4374} + \frac{626\zeta(3)^2}{81} + \frac{84818\zeta(5)}{729} + \frac{539\zeta(7)}{9} + \frac{2080479877}{68024448} - \frac{47369\pi^4}{174960} + \frac{25\pi^6}{15309}$ |
| | $n^{-4}$ | $-\frac{1694161\zeta(3)}{4374} + \frac{3089\zeta(3)^2}{81} - \frac{508\zeta(5)}{27} - \frac{2450\zeta(7)}{9} - \frac{7400332843}{8503056} - \frac{2213\pi^4}{7290} + \frac{305\pi^6}{30618}$ |
| | $n^{-5}$ | $-\frac{1239931\zeta(3)}{1458} - \frac{2834\zeta(3)^2}{81} + \frac{107902\zeta(5)}{729} + \frac{1225\zeta(7)}{3} + \frac{43137004355}{8503056} + \frac{56137\pi^4}{43740} - \frac{445\pi^6}{15309}$ |
| | $n^{-6}$ | $\frac{9044242\zeta(3)}{2187} - 112\zeta(3)^2 - \frac{579260\zeta(5)}{729} - \frac{1078\zeta(7)}{9} - \frac{14088835643}{1062882} - \frac{1802\pi^4}{2187}$ |
| | $n^{-7}$ | $-\frac{3678896\zeta(3)}{729} + \frac{3136\zeta(3)^2}{27} + \frac{16960\zeta(5)}{27} + \frac{9496212881}{531441}$ |
| | $n^{-8}$ | $\frac{4404512\zeta(3)}{2187} - \frac{6468340480}{531441}$ |
| | $n^{-9}$ | $\frac{1767467744}{531441}$ |
| $C_{g_1}^{(6)}$ | | |
| | $n^{-1}$ | $-\frac{488\zeta(3,5)}{81} - \frac{41\pi^4\zeta(3)}{4050} + \frac{222911\zeta(3)}{787320} + \frac{16337\pi^8}{4592700} - \frac{163\pi^6}{76545} + \frac{6263\pi^4}{1749600} + \frac{17743783}{3061100160}$ <br> $-\frac{24893\zeta(3)^2}{10935} - \frac{512\zeta(3)^3}{243} - \frac{73207\zeta(5)}{98415} - \frac{1472\zeta(3)\zeta(5)}{243} + \frac{12241\zeta(7)}{2430} - \frac{92224\zeta(9)}{2187}$ |
| | $n^{-2}$ | $\frac{15512\zeta(3,5)}{675} - \frac{137\pi^4\zeta(3)}{2430} - \frac{9018811\zeta(3)}{4723920} - \frac{69617\pi^8}{5467500} - \frac{27109\pi^6}{590490} - \frac{2114569\pi^4}{47239200} - \frac{1217148265}{1224440064}$ <br> $+\frac{3544\zeta(3)^2}{729} + \frac{704\zeta(3)^3}{81} + \frac{504596\zeta(5)}{32805} + \frac{5240\zeta(3)\zeta(5)}{81} + \frac{163312\zeta(7)}{1215} + \frac{129832\zeta(9)}{729}$ |
| | $n^{-3}$ | $-\frac{7816\zeta(3,5)}{135} + \frac{86\pi^4\zeta(3)}{675} - \frac{214993759\zeta(3)}{1574640} + \frac{200797\pi^8}{7654500} + \frac{21689\pi^6}{137781} + \frac{3206549\pi^4}{2624400} + \frac{4931775043}{136048896}$ <br> $-\frac{364078\zeta(3)^2}{3645} - \frac{5056\zeta(3)^3}{243} - \frac{86601683\zeta(5)}{196830} - \frac{40760\zeta(3)\zeta(5)}{243} - \frac{922984\zeta(7)}{1215} - \frac{950024\zeta(9)}{2187}$ |
| | $n^{-4}$ | $\frac{375328\zeta(3,5)}{2025} + \frac{9827\pi^4\zeta(3)}{18225} + \frac{4722248167\zeta(3)}{2361960} - \frac{2703409\pi^8}{28704375} - \frac{7645\pi^6}{118098} - \frac{27487903\pi^4}{7873200} + \frac{51174486899}{102036672}$ <br> $+\frac{1551302\zeta(3)^2}{10935} + \frac{1472\zeta(3)^3}{27} + \frac{49060643\zeta(5)}{39366} + \frac{352\zeta(3)\zeta(5)}{3} + \frac{741740\zeta(7)}{243} + \frac{280264\zeta(9)}{243}$ |
| | | Continued on next page |

Table 5 Coefficients of $\varepsilon$ expansion for $g_1^*$

| Coef. | | Value |
|---|---|---|
| | $n^{-5}$ | $-\frac{58616\zeta(3,5)}{675}-\frac{1034\pi^4\zeta(3)}{2025}-\frac{570626887\zeta(3)}{118098}+\frac{3437867\pi^8}{38272500}+\frac{865897\pi^6}{4133430}-\frac{54563839\pi^4}{11809800}-\frac{5491876647901}{510183360}$ $+\frac{3981661\zeta(3)^2}{3645}+\frac{64\zeta(3)^3}{27}-\frac{25984307\zeta(5)}{98415}+\frac{15248\zeta(3)\zeta(5)}{81}-\frac{26513393\zeta(7)}{2430}-\frac{42568\zeta(9)}{243}$ |
| | $n^{-6}$ | $-\frac{41104\zeta(3,5)}{135}-\frac{1064\pi^4\zeta(3)}{675}-\frac{2708590031\zeta(3)}{196830}+\frac{31547\pi^8}{546750}-\frac{633328\pi^6}{688905}+\frac{734845\pi^4}{26244}+\frac{1387268404501}{21257640}$ $-\frac{16323208\zeta(3)^2}{10935}-\frac{3712\zeta(3)^3}{27}+\frac{223170298\zeta(5)}{98415}-\frac{187712\zeta(3)\zeta(5)}{243}+\frac{4797416\zeta(7)}{243}-\frac{572528\zeta(9)}{243}$ |
| | $n^{-7}$ | $\frac{94208\zeta(3,5)}{405}+\frac{5936\pi^4\zeta(3)}{3645}+\frac{4686542119\zeta(3)}{59049}-\frac{341504\pi^8}{5740875}+\frac{41870\pi^6}{59049}-\frac{6913691\pi^4}{196830}-\frac{1254411900755}{6377292}$ $-\frac{2940724\zeta(3)^2}{729}+\frac{20992\zeta(3)^3}{243}-\frac{323872688\zeta(5)}{19683}+\frac{125824\zeta(3)\zeta(5)}{81}-\frac{399448\zeta(7)}{27}+\frac{3248960\zeta(9)}{2187}$ |
| | $n^{-8}$ | $-\frac{8165900456\zeta(3)}{59049}+\frac{6267296\zeta(3)^2}{729}+\frac{491993320\zeta(5)}{19683}-\frac{31360\zeta(3)\zeta(5)}{27}+\frac{799876\zeta(7)}{243}+\frac{534966007856}{1594323}+\frac{4168556\pi^4}{295245}$ |
| | $n^{-9}$ | $\frac{2111079040\zeta(3)}{19683}-\frac{9307648\zeta(3)^2}{2187}-\frac{25168640\zeta(5)}{2187}-\frac{175615752704}{531441}$ |
| | $n^{-10}$ | $\frac{840547631840}{4782969}-\frac{1867513088\zeta(3)}{59049}$ |
| | $n^{-11}$ | $-\frac{187351580864}{4782969}$ |

Table 6: Coefficients of $\varepsilon$ expansion for $g_2^*$

| **Coef.** | | **Value** |
|---|---|---|
| $C_{g_2}^{(3)}$ | | |
| | $n^0$ | $\frac{709}{17496}-\frac{4\zeta(3)}{27}$ |
| | $n^{-1}$ | $\frac{11713}{17496}-\frac{32\zeta(3)}{27}$ |
| | $n^{-2}$ | $\frac{80\zeta(3)}{27}+\frac{90281}{8748}$ |
| | $n^{-3}$ | $\frac{16\zeta(3)}{3}-\frac{123707}{2187}$ |
| | $n^{-4}$ | $\frac{187528}{2187}-\frac{224\zeta(3)}{27}$ |
| | $n^{-5}$ | $-\frac{89888}{2187}$ |
| $C_{g_2}^{(4)}$ | | |
| | $n^0$ | $-\frac{106\zeta(3)}{729}+\frac{40\zeta(5)}{81}+\frac{10909}{944784}-\frac{\pi^4}{1215}$ |
| | $n^{-1}$ | $-\frac{56\zeta(3)}{81}+\frac{280\zeta(5)}{81}-\frac{511435}{944784}-\frac{14\pi^4}{1215}$ |
| | $n^{-2}$ | $-\frac{10450\zeta(3)}{729}-\frac{80\zeta(5)}{9}+\frac{406721}{157464}+\frac{32\pi^4}{1215}$ |
| | $n^{-3}$ | $\frac{2704\zeta(3)}{81}-\frac{440\zeta(5)}{81}+\frac{11944655}{118098}+\frac{14\pi^4}{405}$ |
| | $n^{-4}$ | $\frac{23752\zeta(3)}{243}-\frac{400\zeta(5)}{27}-\frac{35478331}{59049}-\frac{68\pi^4}{1215}$ |
| | $n^{-5}$ | $-\frac{200768\zeta(3)}{729}+\frac{320\zeta(5)}{9}+\frac{25018256}{19683}$ |
| | $n^{-6}$ | $\frac{118720\zeta(3)}{729}-\frac{69389720}{59049}$ |
| | $n^{-7}$ | $\frac{23820320}{59049}$ |
| $C_{g_2}^{(5)}$ | | |
| | $n^0$ | $-\frac{11221\zeta(3)}{104976}+\frac{11\zeta(3)^2}{81}+\frac{373\zeta(5)}{729}-\frac{49\zeta(7)}{27}-\frac{321451}{408146688}-\frac{443\pi^4}{524880}+\frac{5\pi^6}{10206}$ |
| | $n^{-1}$ | $\frac{10361\zeta(3)}{104976}+\frac{85\zeta(3)^2}{81}+\frac{1628\zeta(5)}{729}-\frac{98\zeta(7)}{9}+\frac{4069429}{45349632}-\frac{323\pi^4}{87480}+\frac{55\pi^6}{10206}$ |
| | $n^{-2}$ | $\frac{64261\zeta(3)}{26244}+\frac{10\zeta(3)^2}{3}+\frac{29770\zeta(5)}{729}+\frac{980\zeta(7)}{27}-\frac{264392957}{22674816}-\frac{72941\pi^4}{524880}-\frac{205\pi^6}{15309}$ |
| | $n^{-3}$ | $-\frac{1176529\zeta(3)}{6561}-\frac{365\zeta(3)^2}{81}-\frac{83693\zeta(5)}{729}-\frac{2254\zeta(7)}{27}+\frac{256333871}{17006112}+\frac{7747\pi^4}{21870}-\frac{85\pi^6}{30618}$ |
| | $n^{-4}$ | $\frac{4840987\zeta(3)}{13122}-\frac{4354\zeta(3)^2}{81}-\frac{10202\zeta(5)}{729}+\frac{3626\zeta(7)}{9}+\frac{3132906331}{2834352}+\frac{8347\pi^4}{14580}-\frac{305\pi^6}{15309}$ |
| | $n^{-5}$ | $\frac{10668718\zeta(3)}{6561}+\frac{712\zeta(3)^2}{27}-\frac{202864\zeta(5)}{729}-\frac{14896\zeta(7)}{27}-\frac{5033294725}{708588}-\frac{62731\pi^4}{32805}+\frac{620\pi^6}{15309}$ |
| | $n^{-6}$ | $-\frac{40407016\zeta(3)}{6561}+\frac{13888\zeta(3)^2}{81}+\frac{845200\zeta(5)}{729}+\frac{4312\zeta(7)}{27}+\frac{9923276525}{531441}+\frac{37736\pi^4}{32805}$ |
| | $n^{-7}$ | $\frac{46032704\zeta(3)}{6561}-\frac{12544\zeta(3)^2}{81}-\frac{67840\zeta(5)}{81}-\frac{4398801284}{177147}$ |
| | $n^{-8}$ | $\frac{2937809504}{177147}-\frac{17618048\zeta(3)}{6561}$ |
| | $n^{-9}$ | $-\frac{7069870976}{1594323}$ |
| $C_{g_2}^{(6)}$ | | |
| | $n^0$ | $\frac{5776\zeta(3,5)}{6075}+\frac{19\pi^4\zeta(3)}{10935}-\frac{18707\zeta(3)}{7085880}-\frac{88181\pi^8}{172226250}+\frac{1117\pi^6}{2066715}-\frac{19243\pi^4}{28343520}+\frac{32174329}{9183300480}$ |
| | | $+\frac{22429\zeta(3)^2}{32805}+\frac{256\zeta(3)^3}{729}+\frac{63481\zeta(5)}{590490}+\frac{448\zeta(3)\zeta(5)}{729}-\frac{7946\zeta(7)}{3645}+\frac{46112\zeta(9)}{6561}$ |
| | $n^{-1}$ | $\frac{34064\zeta(3,5)}{6075}+\frac{904\pi^4\zeta(3)}{54675}-\frac{10110911\zeta(3)}{14171760}-\frac{663709\pi^8}{172226250}+\frac{5324\pi^6}{2066715}+\frac{39503\pi^4}{28343520}-\frac{104175929}{3673320192}$ |
| | | $+\frac{10466\zeta(3)^2}{10935}+\frac{1280\zeta(3)^3}{729}+\frac{40549\zeta(5)}{65610}+\frac{512\zeta(3)\zeta(5)}{243}-\frac{8303\zeta(7)}{1215}+\frac{230560\zeta(9)}{6561}$ |
| | $n^{-2}$ | $-\frac{44528\zeta(3,5)}{2025}+\frac{3643\pi^4\zeta(3)}{54675}+\frac{246270359\zeta(3)}{14171760}+\frac{770443\pi^8}{57408750}+\frac{31\pi^6}{486}+\frac{3723637\pi^4}{70858800}+\frac{83902290671}{18366600960}$ |

Continued on next page

Table 6 Coefficients of $\varepsilon$ expansion for $g_2^*$

| Coef. | | Value |
|---|---|---|
| | $n^{-3}$ | $+\frac{29359\zeta(3)^2}{6561}-\frac{640\zeta(3)^3}{81}-\frac{4738723\zeta(5)}{590490}-\frac{14192\zeta(3)\zeta(5)}{243}-\frac{510218\zeta(7)}{3645}-\frac{118640\zeta(9)}{729}$ $\frac{95696\zeta(3,5)}{1215}-\frac{653\pi^4\zeta(3)}{6075}+\frac{131677343\zeta(3)}{1417176}-\frac{1295761\pi^8}{34445250}-\frac{817541\pi^6}{4133430}-\frac{25530197\pi^4}{14171760}-\frac{128209072321}{765275040}$ |
| | $n^{-4}$ | $+\frac{3097363\zeta(3)^2}{32805}+\frac{19840\zeta(3)^3}{729}+\frac{90308153\zeta(5)}{196830}+\frac{134768\zeta(3)\zeta(5)}{729}+\frac{1073072\zeta(7)}{1215}+\frac{3712784\zeta(9)}{6561}$ $-\frac{61024\zeta(3,5)}{243}-\frac{44234\pi^4\zeta(3)}{54675}-\frac{2058135142\zeta(3)}{885735}+\frac{471259\pi^8}{3444525}+\frac{15913\pi^6}{196830}+\frac{32403647\pi^4}{7085880}+\frac{157585425307}{1530550080}$ |
| | $n^{-5}$ | $-\frac{1404107\zeta(3)^2}{32805}-\frac{52096\zeta(3)^3}{729}-\frac{312931229\zeta(5)}{295245}-\frac{106496\zeta(3)\zeta(5)}{729}-\frac{39356\zeta(7)}{9}-\frac{9982544\zeta(9)}{6561}$ $\frac{137584\zeta(3,5)}{2025}+\frac{25256\pi^4\zeta(3)}{54675}+\frac{7746961273\zeta(3)}{1771470}-\frac{6507779\pi^8}{57408750}-\frac{10442\pi^6}{25515}+\frac{6249835\pi^4}{708588}+\frac{4976609564287}{382637520}$ |
| | $n^{-6}$ | $-\frac{17009552\zeta(3)^2}{10935}-\frac{5504\zeta(3)^3}{243}-\frac{151805752\zeta(5)}{295245}-\frac{211552\zeta(3)\zeta(5)}{729}+\frac{1294267\zeta(7)}{81}-\frac{259600\zeta(9)}{2187}$ $\frac{2699104\zeta(3,5)}{6075}+\frac{135664\pi^4\zeta(3)}{54675}+\frac{4664802805\zeta(3)}{177147}-\frac{7330087\pi^8}{86113125}+\frac{961046\pi^6}{688905}-\frac{378184379\pi^4}{8857350}-\frac{8577132752053}{95659380}$ |
| | $n^{-7}$ | $+\frac{42371948\zeta(3)^2}{32805}+\frac{143104\zeta(3)^3}{729}-\frac{1144453352\zeta(5)}{295245}+\frac{897728\zeta(3)\zeta(5)}{729}-\frac{100897274\zeta(7)}{3645}+\frac{22087328\zeta(9)}{6561}$ $-\frac{376832\zeta(3,5)}{1215}-\frac{4928\pi^4\zeta(3)}{2187}-\frac{21377118524\zeta(3)}{177147}+\frac{1366016\pi^8}{17222625}-\frac{404920\pi^6}{413343}+\frac{44751454\pi^4}{885735}+\frac{1320431424241}{4782969}$ |
| | $n^{-8}$ | $+\frac{44383216\zeta(3)^2}{6561}-\frac{83968\zeta(3)^3}{729}+\frac{1464733792\zeta(5)}{59049}-\frac{1668608\zeta(3)\zeta(5)}{729}+\frac{14557312\zeta(7)}{729}-\frac{12995840\zeta(9)}{6561}$ $\frac{34952671264\zeta(3)}{177147}-\frac{79942912\zeta(3)^2}{6561}-\frac{689074400\zeta(5)}{19683}+\frac{125440\zeta(3)\zeta(5)}{81}-\frac{3199504\zeta(7)}{729}-\frac{2243022590816}{4782969}-\frac{3460688\pi^4}{177147}$ |
| | $n^{-9}$ | $-\frac{2898667520\zeta(3)}{19683}+\frac{37230592\zeta(3)^2}{6561}+\frac{100674560\zeta(5)}{6561}+\frac{6541580379488}{14348907}$ |
| | $n^{-10}$ | $\frac{7470052352\zeta(3)}{177147}-\frac{3422284430656}{14348907}$ |
| | $n^{-11}$ | $\frac{749406323456}{14348907}$ |

Table 7: Coefficients of RG expansion for $\omega_1$

| **Coef.** | | **Value** |
|---|---|---|
| $C^{(1)}_{\omega_1}$ | | |
| | $n^0$ | $1$ |
| $C^{(2)}_{\omega_1}(n+2)^1$ | | |
| | $n^{-2}$ | $\frac{212}{27}$ |
| | $n^{-1}$ | $-8$ |
| | $n^0$ | $\frac{7}{9}$ |
| | $n^1$ | $-\frac{17}{27}$ |
| $C^{(3)}_{\omega_1}(n+2)^3$ | | |
| | $n^{-4}$ | $-\frac{179776}{729}$ |
| | $n^{-3}$ | $\frac{27616}{729}-\frac{896\zeta(3)}{9}$ |
| | $n^{-2}$ | $\frac{94940}{243}-\frac{704\zeta(3)}{9}$ |
| | $n^{-1}$ | $\frac{160\zeta(3)}{3}-\frac{223660}{729}$ |
| | $n^0$ | $48\zeta(3)+\frac{34522}{729}$ |
| | $n^1$ | $\frac{32\zeta(3)}{9}+\frac{8002}{243}$ |
| | $n^2$ | $-\frac{11683}{2916}$ |
| | $n^3$ | $\frac{8\zeta(3)}{9}+\frac{1603}{2916}$ |
| $C^{(4)}_{\omega_1}(n+2)^5$ | | |
| | $n^{-6}$ | $\frac{190562560}{19683}$ |
| | $n^{-5}$ | $\frac{1519616\zeta(3)}{243}+\frac{30107392}{19683}$ |
| | $n^{-4}$ | $\frac{170240\zeta(3)}{27}+2560\zeta(5)-\frac{350628080}{19683}$ |
| | $n^{-3}$ | $-\frac{1583744\zeta(3)}{243}+5120\zeta(5)-\frac{52778104}{6561}-\frac{448\pi^4}{135}$ |
| | $n^{-2}$ | $-\frac{1944128\zeta(3)}{243}+\frac{33920\zeta(5)}{9}+\frac{189386912}{6561}-\frac{160\pi^4}{27}$ |
| | $n^{-1}$ | $\frac{544288\zeta(3)}{243}-\frac{1280\zeta(5)}{9}-\frac{86039590}{6561}-\frac{224\pi^4}{135}$ |
| | $n^0$ | $\frac{743536\zeta(3)}{243}-\frac{19360\zeta(5)}{9}-\frac{7733252}{6561}+\frac{368\pi^4}{135}$ |
| | $n^1$ | $-\frac{87608\zeta(3)}{243}-\frac{11840\zeta(5)}{9}+\frac{20839757}{13122}+\frac{292\pi^4}{135}$ |
| | $n^2$ | $-\frac{120572\zeta(3)}{243}-\frac{760\zeta(5)}{3}-\frac{1372118}{6561}+\frac{14\pi^4}{27}$ |
| | $n^3$ | $-\frac{2786\zeta(3)}{243}-\frac{80\zeta(5)}{9}-\frac{10660727}{157464}+\frac{8\pi^4}{135}$ |
| | $n^4$ | $\frac{3008\zeta(3)}{243}-\frac{40\zeta(5)}{3}+\frac{1551623}{314928}+\frac{4\pi^4}{135}$ |
| | $n^5$ | $-\frac{158\zeta(3)}{243}-\frac{40\zeta(5)}{9}-\frac{178417}{314928}+\frac{\pi^4}{135}$ |
| $C^{(5)}_{\omega_1}(n+2)^7$ | | |
| | $n^{-8}$ | $-\frac{226235871232}{531441}$ |
| | $n^{-7}$ | $-\frac{805396480\zeta(3)}{2187}-\frac{29448747008}{177147}$ |
| | $n^{-6}$ | $-\frac{986021888\zeta(3)}{2187}-\frac{802816\zeta(3)^2}{27}-\frac{15196160\zeta(5)}{81}+\frac{6175665664}{6561}$ |
| Continued on next page | | |

Table 7 Coefficients of RG expansion for $\omega_1$

| Coef. | | Value |
|---|---|---|
| | $n^{-5}$ | $\frac{1012129792\zeta(3)}{2187} - \frac{229376\zeta(3)^2}{3} - \frac{35338240\zeta(5)}{81} + \frac{351098037248}{531441} + \frac{759808\pi^4}{3645} + \frac{551936\zeta(7)}{9}$ |
| | $n^{-4}$ | $\frac{2034908416\zeta(3)}{2187} - \frac{490496\zeta(3)^2}{9} - \frac{158084365264}{177147} + \frac{1525888\pi^4}{3645} + \frac{2560\pi^6}{189} - \frac{142781440\zeta(5)}{729} - \frac{175616\zeta(7)}{9}$ |
| | $n^{-3}$ | $-\frac{205488256\zeta(3)}{2187} + \frac{302080\zeta(3)^2}{9} - \frac{90520143256}{59049} + \frac{1216\pi^4}{27} + \frac{2560\pi^6}{63} + \frac{164252672\zeta(5)}{729} - \frac{815360\zeta(7)}{3}$ |
| | $n^{-2}$ | $-\frac{1548959680\zeta(3)}{2187} + \frac{1793536\zeta(3)^2}{27} + \frac{1068986488244}{531441} - \frac{1572416\pi^4}{3645} + \frac{85760\pi^6}{1701} + \frac{206505472\zeta(5)}{729} - \frac{934528\zeta(7)}{3}$ |
| | $n^{-1}$ | $-\frac{33034304\zeta(3)}{729} + \frac{478976\zeta(3)^2}{27} - \frac{30319407652}{59049} - \frac{299296\pi^4}{1215} + \frac{14720\pi^6}{567} + \frac{194048\zeta(5)}{3} - \frac{868672\zeta(7)}{9}$ |
| | $n^{0}$ | $\frac{166630688\zeta(3)}{729} - \frac{166400\zeta(3)^2}{9} - \frac{3895339874}{19683} + \frac{14848\pi^4}{135} - \frac{12160\pi^6}{1701}$ $\frac{214816\zeta(7)}{3} - \frac{6727424\zeta(5)}{81}$ |
| | $n^{1}$ | $\frac{14777648\zeta(3)}{729} - \frac{303296\zeta(3)^2}{27} + \frac{48795552835}{531441} + \frac{8800\pi^4}{81} - \frac{31520\pi^6}{1701}$ $\frac{776944\zeta(7)}{9} - \frac{12949952\zeta(5)}{243}$ |
| | $n^{2}$ | $-\frac{65249000\zeta(3)}{2187} + \frac{9632\zeta(3)^2}{27} + \frac{1378075123}{354294} - \frac{3716\pi^4}{1215} - \frac{6320\pi^6}{567} + \frac{1257088\zeta(5)}{243} + \frac{364952\zeta(7)}{9}$ |
| | $n^{3}$ | $-\frac{2894200\zeta(3)}{2187} + \frac{36880\zeta(3)^2}{27} - \frac{69053239}{19683} - \frac{538\pi^4}{27} - \frac{760\pi^6}{243} + \frac{2785672\zeta(5)}{243} + \frac{28616\zeta(7)}{3}$ |
| | $n^{4}$ | $\frac{3951773\zeta(3)}{2187} + \frac{2836\zeta(3)^2}{27} + \frac{2039199229}{8503056} - \frac{29921\pi^4}{7290} - \frac{110\pi^6}{243} + \frac{20252\zeta(5)}{9} + \frac{8624\zeta(7)}{9}$ |
| | $n^{5}$ | $\frac{580243\zeta(3)}{4374} - \frac{2296\zeta(3)^2}{27} + \frac{331662863}{5668704} + \frac{4307\pi^4}{14580} - \frac{20\pi^6}{189}$ $\frac{1960\zeta(7)}{9} - \frac{143288\zeta(5)}{729}$ |
| | $n^{6}$ | $-\frac{85559\zeta(3)}{8748} - \frac{140\zeta(3)^2}{9} - \frac{9425375}{3779136} + \frac{11\pi^4}{135} - \frac{10\pi^6}{243}$ $\frac{392\zeta(7)}{3} - \frac{36128\zeta(5)}{729}$ |
| | $n^{7}$ | $\frac{12349\zeta(3)}{8748} - \frac{4\zeta(3)^2}{9} + \frac{20734249}{34012224} - \frac{79\pi^4}{14580} - \frac{10\pi^6}{1701} + \frac{2324\zeta(5)}{729} + \frac{196\zeta(7)}{9}$ |
| $C^{(6)}_{\omega_1}(n+2)^9$ | | |
| | $n^{-10}$ | $\frac{95924009402368}{4782969}$ |
| | $n^{-9}$ | $\frac{3824666804224\zeta(3)}{177147} + \frac{57233406820352}{4782969}$ |
| | $n^{-8}$ | $\frac{5464539136000\zeta(3)}{177147} + \frac{8339652608\zeta(3)^2}{2187} + \frac{25772687360\zeta(5)}{2187} - \frac{9239684694016}{177147}$ |
| | $n^{-7}$ | $-\frac{1882810683392\zeta(3)}{59049} + \frac{7270989824\zeta(3)^2}{729} + \frac{66187550720\zeta(5)}{2187} - \frac{74743190122496}{1594323} - \frac{80539648\pi^4}{6561} + \frac{4587520\zeta(3)\zeta(5)}{3} - \frac{1287114752\zeta(7)}{243}$ |
| | $n^{-6}$ | $-\frac{48234496\zeta(3,5)}{81} + \frac{174850048\pi^8}{1148175} - \frac{2170880\pi^6}{2187} - \frac{298569728\pi^4}{10935} + \frac{75593202197120}{1594323} - \frac{13716330213376\zeta(3)}{177147} - \frac{802816\pi^4\zeta(3)}{405} + \frac{10822959104\zeta(3)^2}{2187} - \frac{53739520\zeta(3)^3}{243} + \frac{237062809600\zeta(5)}{19683}$ |
| Continued on next page | | |

Table 7 Coefficients of RG expansion for $\omega_1$

| Coef. | | Value |
|---|---|---|
| | | $+\frac{973864960\zeta(3)\zeta(5)}{243}+\frac{149123072\zeta(7)}{243}-\frac{8317337600\zeta(9)}{2187}$ |
| | $n^{-5}$ | $-\frac{236208128\zeta(3,5)}{135}+\frac{943184384\pi^8}{1913625}-\frac{2406400\pi^6}{729}-\frac{87620608\pi^4}{32805}+\frac{15296822474624}{177147}$<br>$-\frac{1412113771520\zeta(3)}{177147}-\frac{573440\pi^4\zeta(3)}{81}-\frac{23791849472\zeta(3)^2}{2187}-\frac{5242880\zeta(3)^3}{9}-\frac{226734792704\zeta(5)}{6561}$<br>$+\frac{878510080\zeta(3)\zeta(5)}{243}+\frac{7317474304\zeta(7)}{243}-\frac{813629440\zeta(9)}{81}$ |
| | $n^{-4}$ | $-\frac{11100160\zeta(3,5)}{9}+\frac{8837888\pi^8}{25515}-\frac{495016960\pi^6}{137781}+\frac{155585152\pi^4}{3645}+\frac{4848503719904}{1594323}$<br>$+\frac{535290640640\zeta(3)}{6561}-\frac{3736576\pi^4\zeta(3)}{405}-\frac{33340307456\zeta(3)^2}{2187}-\frac{21954560\zeta(3)^3}{81}-\frac{656880441344\zeta(5)}{19683}$<br>$+\frac{400015360\zeta(3)\zeta(5)}{243}+\frac{858782720\zeta(7)}{27}-\frac{3025592320\zeta(9)}{729}$ |
| | $n^{-3}$ | $\frac{576053248\zeta(3,5)}{405}-\frac{3261746944\pi^8}{5740875}-\frac{57749504\pi^6}{137781}+\frac{1041226304\pi^4}{32805}-\frac{281901615998096}{1594323}$<br>$+\frac{6127632422528\zeta(3)}{177147}-\frac{360448\pi^4\zeta(3)}{135}-\frac{2280383488\zeta(3)^2}{2187}+\frac{169410560\zeta(3)^3}{243}+\frac{20942412800\zeta(5)}{6561}$<br>$+\frac{43909120\zeta(3)\zeta(5)}{27}-\frac{1643809792\zeta(7)}{243}+\frac{30050590720\zeta(9)}{2187}$ |
| | $n^{-2}$ | $\frac{400728064\zeta(3,5)}{135}-\frac{2286376192\pi^8}{1913625}+\frac{336161792\pi^6}{137781}-\frac{622860416\pi^4}{32805}+\frac{23440380946268}{177147}$<br>$-\frac{8543242526720\zeta(3)}{177147}+\frac{2331904\pi^4\zeta(3)}{405}+\frac{7203772928\zeta(3)^2}{729}+\frac{89620480\zeta(3)^3}{81}+\frac{124459284352\zeta(5)}{6561}$<br>$+\frac{417013760\zeta(3)\zeta(5)}{243}-\frac{6062584832\zeta(7)}{243}+\frac{15487447040\zeta(9)}{729}$ |
| | $n^{-1}$ | $\frac{82302976\zeta(3,5)}{45}-\frac{74749504\pi^8}{91125}+\frac{98779904\pi^6}{45927}-\frac{849717328\pi^4}{32805}-\frac{57965873753804}{4782969}$<br>$-\frac{1085564977888\zeta(3)}{59049}+\frac{833024\pi^4\zeta(3)}{135}+\frac{11797113344\zeta(3)^2}{2187}+\frac{47841280\zeta(3)^3}{81}+\frac{182153230976\zeta(5)}{19683}$<br>$+\frac{41738240\zeta(3)\zeta(5)}{81}-\frac{2376257152\zeta(7)}{243}+\frac{8284528640\zeta(9)}{729}$ |
| | $n^{0}$ | $\frac{4877312\zeta(3,5)}{81}-\frac{105104096\pi^8}{1148175}+\frac{39207808\pi^6}{137781}+\frac{6774616\pi^4}{32805}-\frac{85024975005739}{4782969}$<br>$+\frac{863917294832\zeta(3)}{59049}+\frac{28544\pi^4\zeta(3)}{27}-\frac{3238369792\zeta(3)^2}{2187}-\frac{6430720\zeta(3)^3}{243}-\frac{55041099136\zeta(5)}{19683}$<br>$-\frac{57251840\zeta(3)\zeta(5)}{243}+\frac{284296064\zeta(7)}{81}-\frac{1065436160\zeta(9)}{2187}$ |
| | $n^{1}$ | $-\frac{9187328\zeta(3,5)}{15}+\frac{54377984\pi^8}{212625}-\frac{4179968\pi^6}{6561}+\frac{17314976\pi^4}{2187}+\frac{800089158703}{177147}$<br>$+\frac{700272187856\zeta(3)}{177147}-\frac{227584\pi^4\zeta(3)}{135}-\frac{4223648000\zeta(3)^2}{2187}-\frac{18145280\zeta(3)^3}{81}-\frac{8746152224\zeta(5)}{2187}$<br>$-\frac{19924480\zeta(3)\zeta(5)}{81}+\frac{316242064\zeta(7)}{81}-\frac{3167779840\zeta(9)}{729}$ |
| | $n^{2}$ | $-\frac{6785536\zeta(3,5)}{15}+\frac{47400208\pi^8}{212625}-\frac{16963936\pi^6}{45927}+\frac{10405696\pi^4}{6561}+\frac{1043100732122}{1594323}$<br>$-\frac{121724897104\zeta(3)}{59049}-\frac{46496\pi^4\zeta(3)}{45}-\frac{73310464\zeta(3)^2}{243}-\frac{12692480\zeta(3)^3}{81}-\frac{3327142168\zeta(5)}{6561}$<br>$-\frac{22092800\zeta(3)\zeta(5)}{81}+\frac{238811120\zeta(7)}{243}-\frac{2243171200\zeta(9)}{729}$ |
| | $n^{3}$ | $-\frac{72620224\zeta(3,5)}{405}+\frac{568027822\pi^8}{5740875}+\frac{213992\pi^6}{15309}-\frac{352222\pi^4}{405}-\frac{383400589610}{1594323}$<br>$-\frac{71360608688\zeta(3)}{177147}-\frac{29312\pi^4\zeta(3)}{405}+\frac{263851888\zeta(3)^2}{2187}-\frac{15441920\zeta(3)^3}{243}+\frac{10760498672\zeta(5)}{19683}$<br>$-\frac{64149760\zeta(3)\zeta(5)}{243}-\frac{64211492\zeta(7)}{243}-\frac{2771557120\zeta(9)}{2187}$ |
| | $n^{4}$ | $-\frac{1169696\zeta(3,5)}{27}+\frac{10090013\pi^8}{382725}+\frac{511892\pi^6}{6561}-\frac{15254677\pi^4}{65610}-\frac{7433381435}{708588}$<br>$+\frac{16262289125\zeta(3)}{177147}+\frac{42124\pi^4\zeta(3)}{405}+\frac{37692104\zeta(3)^2}{2187}-\frac{1329920\zeta(3)^3}{81}+\frac{908522840\zeta(5)}{6561}$<br>$-\frac{30452800\zeta(3)\zeta(5)}{243}-\frac{68208820\zeta(7)}{243}-\frac{244148320\zeta(9)}{729}$ |
| | $n^{5}$ | $-\frac{263776\zeta(3,5)}{45}+\frac{2638603\pi^8}{637875}+\frac{3538264\pi^6}{137781}+\frac{2345563\pi^4}{43740}+\frac{20173433257}{25509168}$<br>$+\frac{417130121\zeta(3)}{39366}+\frac{1952\pi^4\zeta(3)}{81}-\frac{25530436\zeta(3)^2}{2187}-\frac{21760\zeta(3)^3}{9}-\frac{520285720\zeta(5)}{19683}$<br>$-\frac{5515840\zeta(3)\zeta(5)}{243}-\frac{6744070\zeta(7)}{81}-\frac{4174880\zeta(9)}{81}$ |

Continued on next page

Table 7 Coefficients of RG expansion for $\omega_1$

| Coef. | | Value |
|---|---|---|
| | $n^6$ | $-\frac{309568\zeta(3,5)}{405}+\frac{517522\pi^8}{820125}+\frac{220076\pi^6}{137781}+\frac{251335\pi^4}{13122}-\frac{20016314209}{102036672}$ $-\frac{346862246\zeta(3)}{177147}-\frac{223\pi^4\zeta(3)}{45}-\frac{6664562\zeta(3)^2}{2187}-\frac{70400\zeta(3)^3}{243}-\frac{126244763\zeta(5)}{13122}$ $+\frac{33760\zeta(3)\zeta(5)}{27}-\frac{1238354\zeta(7)}{243}-\frac{14132320\zeta(9)}{2187}$ |
| | $n^7$ | $-\frac{55456\zeta(3,5)}{135}+\frac{494293\pi^8}{1913625}-\frac{72218\pi^6}{137781}+\frac{433823\pi^4}{524880}+\frac{88506139}{11337408}$ $-\frac{171378221\zeta(3)}{1417176}-\frac{1006\pi^4\zeta(3)}{405}-\frac{244684\zeta(3)^2}{729}-\frac{1280\zeta(3)^3}{9}-\frac{3019253\zeta(5)}{13122}$ $+\frac{150880\zeta(3)\zeta(5)}{243}+\frac{486368\zeta(7)}{243}-\frac{235040\zeta(9)}{81}$ |
| | $n^8$ | $-\frac{1184\zeta(3,5)}{9}+\frac{9437\pi^8}{127575}-\frac{2398\pi^6}{45927}-\frac{36163\pi^4}{1049760}+\frac{4224103957}{1224440064}$ $+\frac{259177\zeta(3)}{944784}-\frac{13\pi^4\zeta(3)}{45}-\frac{138212\zeta(3)^2}{2187}-\frac{1280\zeta(3)^3}{27}+\frac{2382389\zeta(5)}{39366}$ $-\frac{640\zeta(3)\zeta(5)}{9}+\frac{57943\zeta(7)}{243}-\frac{230560\zeta(9)}{243}$ |
| | $n^9$ | $-\frac{5776\zeta(3,5)}{405}+\frac{88181\pi^8}{11481750}+\frac{1081\pi^6}{275562}+\frac{12349\pi^4}{1049760}-\frac{853678429}{1224440064}$ $-\frac{6886777\zeta(3)}{2834352}-\frac{\pi^4\zeta(3)}{135}-\frac{16904\zeta(3)^2}{2187}-\frac{1280\zeta(3)^3}{243}-\frac{95713\zeta(5)}{39366}$ $-\frac{4960\zeta(3)\zeta(5)}{243}-\frac{961\zeta(7)}{81}-\frac{230560\zeta(9)}{2187}$ |

Table 8: Coefficients of RG expansion for $\omega_2$

| **Coef.** | | **Value** |
|---|---|---|
| $C^{(1)}_{\omega_2}$ | | |
| | $n^{-1}$ | $-\frac{4}{3}$ |
| | $n^{0}$ | $\frac{1}{3}$ |
| $C^{(2)}_{\omega_2}(n+2)$ | | |
| | $n^{-3}$ | $\frac{848}{81}$ |
| | $n^{-2}$ | $-\frac{1508}{81}$ |
| | $n^{-1}$ | $\frac{196}{27}$ |
| | $n^{0}$ | $\frac{91}{81}$ |
| | $n^{1}$ | $-\frac{19}{81}$ |
| $C^{(3)}_{\omega_2}(n+2)^3$ | | |
| | $n^{-5}$ | $-\frac{719104}{2187}$ |
| | $n^{-4}$ | $\frac{1154240}{2187} - \frac{1792\zeta(3)}{27}$ |
| | $n^{-3}$ | $\frac{362000}{2187} - \frac{256\zeta(3)}{9}$ |
| | $n^{-2}$ | $\frac{2752\zeta(3)}{27} - \frac{1382284}{2187}$ |
| | $n^{-1}$ | $\frac{352\zeta(3)}{9} + \frac{571484}{2187}$ |
| | $n^{0}$ | $\frac{54338}{2187} - \frac{896\zeta(3)}{27}$ |
| | $n^{1}$ | $-\frac{376\zeta(3)}{27} - \frac{44599}{2187}$ |
| | $n^{2}$ | $\frac{16\zeta(3)}{27} + \frac{16637}{8748}$ |
| | $n^{3}$ | $\frac{8\zeta(3)}{27} - \frac{937}{8748}$ |
| $C^{(4)}_{\omega_2}(n+2)^5$ | | |
| | $n^{-7}$ | $\frac{762250240}{59049}$ |
| | $n^{-6}$ | $\frac{3799040\zeta(3)}{729} - \frac{363825920}{19683}$ |
| | $n^{-5}$ | $\frac{547840\zeta(3)}{729} + \frac{10240\zeta(5)}{9} - \frac{13118272}{729}$ |
| | $n^{-4}$ | $-\frac{8527616\zeta(3)}{729} + \frac{89600\zeta(5)}{81} + \frac{1719557552}{59049} - \frac{896\pi^4}{405}$ |
| | $n^{-3}$ | $-\frac{705664\zeta(3)}{243} + \frac{33280\zeta(5)}{81} + \frac{111592664}{6561} - \frac{256\pi^4}{81}$ |
| | $n^{-2}$ | $\frac{81280\zeta(3)}{9} - \frac{92800\zeta(5)}{81} - \frac{75041320}{2187} + \frac{256\pi^4}{135}$ |
| | $n^{-1}$ | $\frac{196064\zeta(3)}{81} - \frac{53120\zeta(5)}{27} + \frac{208697738}{19683} + \frac{1808\pi^4}{405}$ |
| | $n^{0}$ | $-\frac{197056\zeta(3)}{81} - \frac{40160\zeta(5)}{81} + \frac{15685726}{6561} + \frac{424\pi^4}{405}$ |
| | $n^{1}$ | $-\frac{146728\zeta(3)}{243} + \frac{47840\zeta(5)}{81} - \frac{5675003}{4374} - \frac{56\pi^4}{45}$ |
| | $n^{2}$ | $\frac{47408\zeta(3)}{243} + \frac{3080\zeta(5)}{9} + \frac{3466459}{118098} - \frac{292\pi^4}{405}$ |
| | $n^{3}$ | $\frac{22606\zeta(3)}{729} + \frac{2560\zeta(5)}{81} + \frac{4943401}{157464} - \frac{7\pi^4}{81}$ |
| | $n^{4}$ | $-\frac{1789\zeta(3)}{729} - \frac{760\zeta(5)}{81} - \frac{122071}{34992} + \frac{2\pi^4}{135}$ |
| | $n^{5}$ | $\frac{119\zeta(3)}{729} - \frac{80\zeta(5)}{81} - \frac{24857}{944784} + \frac{\pi^4}{405}$ |

Continued on next page

Table 8 Coefficients of $\epsilon$ expansion for $\omega_2$

| Coef. | | Value |
|---|---|---|
| $C^{(5)}_{\omega_2}(n+2)^7$ | | |
| | $n^{-9}$ | $-\frac{904943484928}{1594323}$ |
| | $n^{-8}$ | $\frac{1139072241664}{1594323}-\frac{2255110144\zeta(3)}{6561}$ |
| | $n^{-7}$ | $-\frac{273547264\zeta(3)}{6561}-\frac{1605632\zeta(3)^2}{81}-\frac{8683520\zeta(5)}{81}+\frac{668195317760}{531441}$ |
| | $n^{-6}$ | $\frac{701937664\zeta(3)}{729}-\frac{3153920\zeta(3)^2}{81}-\frac{242739200\zeta(5)}{2187}-\frac{2257643603968}{1594323}+\frac{379904\pi^4}{2187}$ $+\frac{551936\zeta(7)}{27}$ |
| | $n^{-5}$ | $\frac{718615552\zeta(3)}{2187}+\frac{753664\zeta(3)^2}{81}-\frac{2514275344448}{1594323}+\frac{144896\pi^4}{729}+\frac{10240\pi^6}{1701}$ $+\frac{91197440\zeta(5)}{729}-\frac{175616\zeta(7)}{3}$ |
| | $n^{-4}$ | $-\frac{7295334656\zeta(3)}{6561}+\frac{6151168\zeta(3)^2}{81}+\frac{644265436624}{531441}-\frac{3515008\pi^4}{10935}+\frac{181760\pi^6}{15309}$ $+\frac{447378944\zeta(5)}{2187}-\frac{2834944\zeta(7)}{27}$ |
| | $n^{-3}$ | $-\frac{349319296\zeta(3)}{729}+\frac{1117184\zeta(3)^2}{27}+\frac{3138908400344}{1594323}-\frac{5253824\pi^4}{10935}+\frac{48640\pi^6}{5103}$ $+\frac{61357568\zeta(5)}{729}+\frac{238336\zeta(7)}{27}$ |
| | $n^{-2}$ | $\frac{4217377984\zeta(3)}{6561}-37376\zeta(3)^2-\frac{3381093084092}{1594323}+\frac{1167392\pi^4}{10935}-\frac{37120\pi^6}{15309}$ $\frac{702464\zeta(7)}{9}-\frac{61244672\zeta(5)}{729}$ |
| | $n^{-1}$ | $\frac{516558784\zeta(3)}{2187}-\frac{3258112\zeta(3)^2}{81}+\frac{68582687860}{177147}+\frac{1303168\pi^4}{3645}-\frac{81280\pi^6}{5103}$ $\frac{1361024\zeta(7)}{27}-\frac{95629568\zeta(5)}{729}$ |
| | $n^{0}$ | $-\frac{1521568\zeta(3)}{9}-\frac{163072\zeta(3)^2}{81}+\frac{341578511470}{1594323}+\frac{90944\pi^4}{1215}-\frac{74240\pi^6}{5103}$ $\frac{613088\zeta(7)}{27}-\frac{20148032\zeta(5)}{729}$ |
| | $n^{1}$ | $-\frac{296748176\zeta(3)}{6561}+\frac{752192\zeta(3)^2}{81}-\frac{113928189751}{1594323}-\frac{295424\pi^4}{3645}-\frac{10720\pi^6}{5103}$ $+\frac{8353408\zeta(5)}{243}+\frac{74480\zeta(7)}{27}$ |
| | $n^{2}$ | $\frac{119880736\zeta(3)}{6561}+\frac{232576\zeta(3)^2}{81}-\frac{4222320313}{1062882}-\frac{123556\pi^4}{3645}+\frac{1040\pi^6}{243}$ $+\frac{11271560\zeta(5)}{729}-\frac{276556\zeta(7)}{27}$ |
| | $n^{3}$ | $\frac{2003492\zeta(3)}{729}-\frac{18896\zeta(3)^2}{81}+\frac{16653097063}{6377292}+\frac{27392\pi^4}{10935}+\frac{14080\pi^6}{5103}$ $-\frac{2750848\zeta(5)}{2187}-7742\zeta(7)$ |
| | $n^{4}$ | $-\frac{1442003\zeta(3)}{2187}-\frac{13388\zeta(3)^2}{81}-\frac{1597131205}{25509168}+\frac{18791\pi^4}{7290}+\frac{970\pi^6}{1701}$ $-\frac{955454\zeta(5)}{729}-\frac{48412\zeta(7)}{27}$ |
| | $n^{5}$ | $-\frac{298685\zeta(3)}{13122}-\frac{656\zeta(3)^2}{81}-\frac{316976663}{17006112}+\frac{7963\pi^4}{43740}-\frac{200\pi^6}{15309}$ $\frac{490\zeta(7)}{9}-\frac{182858\zeta(5)}{2187}$ |
| | $n^{6}$ | $\frac{26383\zeta(3)}{2916}-\frac{4\zeta(3)^2}{81}-\frac{137965547}{102036672}-\frac{1313\pi^4}{87480}-\frac{10\pi^6}{567}$ $+\frac{2540\zeta(5)}{243}+\frac{1666\zeta(7)}{27}$ |
| | $n^{7}$ | $\frac{3335\zeta(3)}{26244}-\frac{16\zeta(3)^2}{81}-\frac{64327}{102036672}+\frac{119\pi^4}{87480}-\frac{20\pi^6}{15309}$ $\frac{98\zeta(7)}{27}-\frac{352\zeta(5)}{729}$ |
| $C^{(6)}_{\omega_2}(n+2)^9$ | | |
| | $n^{-11}$ | $\frac{383696037609472}{14348907}$ |

Continued on next page

Table 8 Coefficients of $\epsilon$ expansion for $\omega_2$

| Coef. | | Value |
|---|---|---|
| | $n^{-10}$ | $\frac{3824666804224\zeta(3)}{177147}-\frac{416513044742144}{14348907}$ |
| | $n^{-9}$ | $\frac{709672828928\zeta(3)}{177147}+\frac{19062063104\zeta(3)^2}{6561}+\frac{51545374720\zeta(5)}{6561}-\frac{1148459085971456}{14348907}$ |
| | $n^{-8}$ | $-\frac{12792854437888\zeta(3)}{177147}+\frac{33865990144\zeta(3)^2}{6561}+\frac{535111843840\zeta(5)}{59049}+\frac{326099343560704}{4782969}-\frac{1127555072\pi^4}{98415}+\frac{64225280\zeta(3)\zeta(5)}{81}-\frac{1638146048\zeta(7)}{729}$ |
| | $n^{-7}$ | $-\frac{192937984\zeta(3,5)}{1215}+\frac{699400192\pi^8}{17222625}-\frac{8683520\pi^6}{15309}-\frac{1264328704\pi^4}{98415}+\frac{590437476587008}{4782969}-\frac{5645889642496\zeta(3)}{177147}-\frac{1605632\pi^4\zeta(3)}{1215}-\frac{28034498560\zeta(3)^2}{6561}-\frac{42991616\zeta(3)^3}{729}-\frac{901226356736\zeta(5)}{59049}+\frac{424542208\zeta(3)\zeta(5)}{243}+\frac{1320833024\zeta(7)}{243}-\frac{6653870080\zeta(9)}{6561}$ |
| | $n^{-6}$ | $-\frac{343851008\zeta(3,5)}{1215}+\frac{1507249664\pi^8}{17222625}-\frac{477194240\pi^6}{413343}+\frac{2740057088\pi^4}{98415}-\frac{279870161475968}{4782969}+\frac{17553307504640\zeta(3)}{177147}-\frac{4759552\pi^4\zeta(3)}{1215}-\frac{96490639360\zeta(3)^2}{6561}-\frac{47054848\zeta(3)^3}{729}-\frac{57006788608\zeta(5)}{2187}+\frac{741638144\zeta(3)\zeta(5)}{729}+\frac{10481601536\zeta(7)}{729}-\frac{7627292672\zeta(9)}{6561}$ |
| | $n^{-5}$ | $\frac{124018688\zeta(3,5)}{405}-\frac{611573504\pi^8}{5740875}-\frac{27760640\pi^6}{413343}+\frac{4202449408\pi^4}{98415}-\frac{651414468338176}{4782969}+\frac{12358651738112\zeta(3)}{177147}-\frac{311296\pi^4\zeta(3)}{135}-\frac{2954719232\zeta(3)^2}{729}+\frac{45154304\zeta(3)^3}{243}+\frac{228325578752\zeta(5)}{59049}-\frac{101974016\zeta(3)\zeta(5)}{243}-\frac{3961292800\zeta(7)}{729}+\frac{7469719552\zeta(9)}{2187}$ |
| | $n^{-4}$ | $\frac{224137216\zeta(3,5)}{243}-\frac{1216721536\pi^8}{3444525}+\frac{220289024\pi^6}{137781}-\frac{1780064128\pi^4}{98415}-\frac{668360034016}{4782969}-\frac{13535216385280\zeta(3)}{177147}+\frac{2038784\pi^4\zeta(3)}{405}+\frac{90713368576\zeta(3)^2}{6561}+\frac{240025600\zeta(3)^3}{729}+\frac{1291859750912\zeta(5)}{59049}-\frac{1168654336\zeta(3)\zeta(5)}{729}-\frac{15337799168\zeta(7)}{729}+\frac{40944693248\zeta(9)}{6561}$ |
| | $n^{-3}$ | $\frac{93636608\zeta(3,5)}{243}-\frac{622152512\pi^8}{3444525}+\frac{100262912\pi^6}{59049}-\frac{4950123328\pi^4}{98415}+\frac{943351903428608}{4782969}-\frac{11399454691456\zeta(3)}{177147}+\frac{9691136\pi^4\zeta(3)}{1215}+\frac{67952373760\zeta(3)^2}{6561}+\frac{26624000\zeta(3)^3}{729}+\frac{663786101248\zeta(5)}{59049}-\frac{1728339968\zeta(3)\zeta(5)}{729}-\frac{3045323776\zeta(7)}{729}+\frac{5150980096\zeta(9)}{6561}$ |
| | $n^{-2}$ | $-\frac{12961792\zeta(3,5)}{27}+\frac{64174912\pi^8}{382725}+\frac{114215552\pi^6}{413343}-\frac{375164672\pi^4}{98415}-\frac{1890254195363900}{14348907}+\frac{6803193506048\zeta(3)}{177147}+\frac{1861888\pi^4\zeta(3)}{1215}-\frac{26746885888\zeta(3)^2}{6561}-\frac{58556416\zeta(3)^3}{243}-\frac{88564094720\zeta(5)}{19683}-\frac{796493824\zeta(3)\zeta(5)}{729}+\frac{6788305856\zeta(7)}{729}-\frac{10114985984\zeta(9)}{2187}$ |
| | $n^{-1}$ | $-\frac{664769536\zeta(3,5)}{1215}+\frac{4076769568\pi^8}{17222625}-\frac{141745664\pi^6}{137781}+\frac{498108592\pi^4}{19683}+\frac{99412553626336}{14348907}+\frac{1498654070368\zeta(3)}{59049}-\frac{1089536\pi^4\zeta(3)}{243}-\frac{1492050688\zeta(3)^2}{243}-\frac{129179648\zeta(3)^3}{729}-\frac{174032772992\zeta(5)}{19683}+\frac{85489664\zeta(3)\zeta(5)}{81}+\frac{3449864512\zeta(7)}{729}-\frac{22754065408\zeta(9)}{6561}$ |
| | $n^{0}$ | $-\frac{250942976\zeta(3,5)}{1215}+\frac{2091371888\pi^8}{17222625}-\frac{44019968\pi^6}{45927}+\frac{747398888\pi^4}{98415}+\frac{247389001288273}{14348907}-\frac{1871825687216\zeta(3)}{177147}-\frac{4178048\pi^4\zeta(3)}{1215}-\frac{3399727360\zeta(3)^2}{6561}-\frac{26324992\zeta(3)^3}{729}-\frac{121465406080\zeta(5)}{59049}+\frac{857664512\zeta(3)\zeta(5)}{729}-\frac{19454048\zeta(7)}{729}-\frac{4605346304\zeta(9)}{6561}$ |
| | $n^{1}$ | $-\frac{3933952\zeta(3,5)}{135}+\frac{68221336\pi^8}{1913625}-\frac{2817280\pi^6}{19683}-\frac{101855216\pi^4}{19683}-\frac{17939603496865}{4782969}-\frac{782360516768\zeta(3)}{177147}-\frac{75136\pi^4\zeta(3)}{405}+\frac{8408932736\zeta(3)^2}{6561}+\frac{63488\zeta(3)^3}{81}+\frac{127499478560\zeta(5)}{59049}+\frac{13439488\zeta(3)\zeta(5)}{243}-\frac{280415632\zeta(7)}{729}+\frac{23725312\zeta(9)}{729}$ |
| | $n^{2}$ | $\frac{22700608\zeta(3,5)}{1215}-\frac{15049942\pi^8}{2460375}+\frac{10410856\pi^6}{45927}-\frac{227086604\pi^4}{98415}-\frac{2584950328600}{4782969}+\frac{240956206384\zeta(3)}{177147}+\frac{188800\pi^4\zeta(3)}{243}+\frac{2207024080\zeta(3)^2}{6561}+\frac{2261504\zeta(3)^3}{729}+\frac{54535170224\zeta(5)}{59049}-\frac{78943616\zeta(3)\zeta(5)}{243}-\frac{73433684\zeta(7)}{243}+\frac{411441856\zeta(9)}{6561}$ |

Continued on next page

Table 8 Coefficients of $\epsilon$ expansion for $\omega_2$

| Coef. | | Value |
|---|---|---|
| | $n^3$ | $\frac{44346272\zeta(3,5)}{1215}-\frac{381398561\pi^8}{17222625}+\frac{50539400\pi^6}{413343}+\frac{6372512\pi^4}{19683}+\frac{846441257411}{4782969}$ $+\frac{53983758028\zeta(3)}{177147}+\frac{401728\pi^4\zeta(3)}{1215}-\frac{517772048\zeta(3)^2}{6561}+\frac{7405312\zeta(3)^3}{729}-\frac{3154133416\zeta(5)}{19683}$ $-\frac{69009152\zeta(3)\zeta(5)}{729}-\frac{168666368\zeta(7)}{729}+\frac{1284155168\zeta(9)}{6561}$ |
| | $n^4$ | $\frac{10727728\zeta(3,5)}{405}-\frac{180650303\pi^8}{11481750}+\frac{3307880\pi^6}{413343}+\frac{43675603\pi^4}{196830}-\frac{12935187434}{4782969}$ $-\frac{11879180387\zeta(3)}{177147}+\frac{1724\pi^4\zeta(3)}{81}-\frac{56827784\zeta(3)^2}{2187}+\frac{2167168\zeta(3)^3}{243}-\frac{6032839280\zeta(5)}{59049}$ $+\frac{8787136\zeta(3)\zeta(5)}{243}-\frac{30794042\zeta(7)}{729}+\frac{382339472\zeta(9)}{2187}$ |
| | $n^5$ | $\frac{10387336\zeta(3,5)}{1215}-\frac{338105317\pi^8}{68890500}-\frac{1198772\pi^6}{137781}+\frac{65011\pi^4}{393660}-\frac{13830663439}{38263752}$ $-\frac{2259249889\zeta(3)}{354294}-\frac{6256\pi^4\zeta(3)}{405}+\frac{22775456\zeta(3)^2}{6561}+\frac{2229056\zeta(3)^3}{729}-\frac{7571258\zeta(5)}{59049}$ $+\frac{16406368\zeta(3)\zeta(5)}{729}+\frac{14309846\zeta(7)}{729}+\frac{398796184\zeta(9)}{6561}$ |
| | $n^6$ | $\frac{951536\zeta(3,5)}{1215}-\frac{15372451\pi^8}{34445250}-\frac{1721101\pi^6}{826686}-\frac{1171483\pi^4}{196830}+\frac{12776619403}{306110016}$ $+\frac{208928119\zeta(3)}{177147}-\frac{4007\pi^4\zeta(3)}{1215}+\frac{6100895\zeta(3)^2}{6561}+\frac{206656\zeta(3)^3}{729}+\frac{146528477\zeta(5)}{59049}$ $+\frac{2083016\zeta(3)\zeta(5)}{729}+\frac{21422029\zeta(7)}{2916}+\frac{37813592\zeta(9)}{6561}$ |
| | $n^7$ | $-\frac{9128\zeta(3,5)}{45}+\frac{40223\pi^8}{364500}-\frac{25409\pi^6}{413343}+\frac{182879\pi^4}{1574640}-\frac{12152882495}{229582512}$ $+\frac{48940037\zeta(3)}{1417176}-\frac{184\pi^4\zeta(3)}{1215}-\frac{626111\zeta(3)^2}{6561}-\frac{18176\zeta(3)^3}{243}-\frac{2085685\zeta(5)}{39366}$ $-\frac{225992\zeta(3)\zeta(5)}{729}+\frac{1153933\zeta(7)}{2916}-\frac{3233632\zeta(9)}{2187}$ |
| | $n^8$ | $-\frac{57512\zeta(3,5)}{1215}+\frac{258047\pi^8}{9841500}+\frac{1364\pi^6}{137781}+\frac{250787\pi^4}{3149280}+\frac{5822674441}{3673320192}$ $+\frac{8809073\zeta(3)}{2834352}-\frac{17\pi^4\zeta(3)}{1215}-\frac{49790\zeta(3)^2}{2187}-\frac{12544\zeta(3)^3}{729}-\frac{1619723\zeta(5)}{78732}$ $-\frac{18464\zeta(3)\zeta(5)}{243}-\frac{33124\zeta(7)}{729}-\frac{2259488\zeta(9)}{6561}$ |
| | $n^9$ | $-\frac{488\zeta(3,5)}{243}+\frac{16337\pi^8}{13778100}-\frac{29\pi^6}{39366}+\frac{667\pi^4}{629856}+\frac{10365955}{3673320192}$ $+\frac{68143\zeta(3)}{944784}-\frac{4\pi^4\zeta(3)}{1215}-\frac{5038\zeta(3)^2}{6561}-\frac{512\zeta(3)^3}{729}-\frac{48077\zeta(5)}{236196}$ $-\frac{1472\zeta(3)\zeta(5)}{729}+\frac{2491\zeta(7)}{1458}-\frac{92224\zeta(9)}{6561}$ |

Table 9: Coefficients of $\varepsilon$ expansion for $\eta$

| **Coef.** | | **Value** |
|---|---|---|
| $C_\eta^{(2)}$ | | |
| | $n^0$ | $\frac{1}{54}$ |
| | $n^{-1}$ | $\frac{1}{54}$ |
| | $n^{-2}$ | $-\frac{1}{27}$ |
| $C_\eta^{(3)}$ | | |
| | $n^0$ | $\frac{109}{5832}$ |
| | $n^{-1}$ | $-\frac{331}{5832}$ |
| | $n^{-2}$ | $\frac{325}{972}$ |
| | $n^{-3}$ | $-\frac{428}{729}$ |
| | $n^{-4}$ | $\frac{212}{729}$ |
| $C_\eta^{(4)}$ | | |
| | $n^0$ | $\frac{7217}{629856} - \frac{4\zeta(3)}{243}$ |
| | $n^{-1}$ | $\frac{20\zeta(3)}{243} + \frac{7205}{209952}$ |
| | $n^{-2}$ | $-\frac{80\zeta(3)}{243} - \frac{11183}{13122}$ |
| | $n^{-3}$ | $\frac{40\zeta(3)}{243} + \frac{350035}{78732}$ |
| | $n^{-4}$ | $\frac{136\zeta(3)}{243} - \frac{244135}{26244}$ |
| | $n^{-5}$ | $\frac{55882}{6561} - \frac{112\zeta(3)}{243}$ |
| | $n^{-6}$ | $-\frac{56180}{19683}$ |
| $C_\eta^{(5)}$ | | |
| | $n^0$ | $-\frac{329\zeta(3)}{17496} + \frac{40\zeta(5)}{729} + \frac{321511}{68024448} - \frac{\pi^4}{7290}$ |
| | $n^{-1}$ | $-\frac{1867\zeta(3)}{17496} - \frac{80\zeta(5)}{243} + \frac{1627189}{68024448} + \frac{\pi^4}{1458}$ |
| | $n^{-2}$ | $\frac{7975\zeta(3)}{4374} + \frac{920\zeta(5)}{729} + \frac{11047633}{17006112} - \frac{2\pi^4}{729}$ |
| | $n^{-3}$ | $-\frac{13760\zeta(3)}{2187} - \frac{680\zeta(5)}{729} - \frac{97259995}{8503056} + \frac{\pi^4}{729}$ |
| | $n^{-4}$ | $\frac{2033\zeta(3)}{729} - \frac{40\zeta(5)}{729} + \frac{507264575}{8503056} + \frac{17\pi^4}{3645}$ |
| | $n^{-5}$ | $\frac{37276\zeta(3)}{2187} - \frac{160\zeta(5)}{81} - \frac{77891743}{531441} - \frac{14\pi^4}{3645}$ |
| | $n^{-6}$ | $-\frac{19024\zeta(3)}{729} + \frac{160\zeta(5)}{81} + \frac{99764570}{531441}$ |
| | $n^{-7}$ | $\frac{23744\zeta(3)}{2187} - \frac{64532800}{531441}$ |
| | $n^{-8}$ | $\frac{16674224}{531441}$ |
| $C_\eta^{(6)}$ | | |
| | $n^0$ | $-\frac{90731\zeta(3)}{5668704} + \frac{38\zeta(3)^2}{2187} + \frac{4577\zeta(5)}{78732} - \frac{49\zeta(7)}{243} + \frac{3421613}{2448880128} - \frac{329\pi^4}{2099520} + \frac{10\pi^6}{137781}$ |
| | $n^{-1}$ | $-\frac{76003\zeta(3)}{1889568} + \frac{80\zeta(3)^2}{2187} + \frac{32015\zeta(5)}{78732} + \frac{343\zeta(7)}{243} - \frac{21814559}{2448880128} - \frac{1867\pi^4}{2099520} - \frac{20\pi^6}{45927}$ |
| | $n^{-2}$ | $-\frac{429148\zeta(3)}{177147} - \frac{62\zeta(3)^2}{81} - \frac{44900\zeta(5)}{6561} - \frac{1372\zeta(7)}{243} + \frac{36424669}{136048896} + \frac{1595\pi^4}{104976} + \frac{230\pi^6}{137781}$ |
| | $n^{-3}$ | $\frac{41844845\zeta(3)}{1417176} + \frac{4142\zeta(3)^2}{2187} + \frac{35905\zeta(5)}{1458} + \frac{686\zeta(7)}{81} + \frac{1070137823}{102036672} - \frac{344\pi^4}{6561} - \frac{170\pi^6}{137781}$ |
| | | Continued on next page |

Table 9 Coefficients of $\varepsilon$ expansion for $\eta$

| Coef. | | Value |
|---|---|---|
| | $n^{-4}$ | $-\frac{3812633\zeta(3)}{39366}+\frac{5758\zeta(3)^2}{2187}-\frac{1087189\zeta(5)}{39366}-\frac{4802\zeta(7)}{243}-\frac{3925669625}{25509168}+\frac{2033\pi^4}{87480}-\frac{10\pi^6}{137781}$ |
| | $n^{-5}$ | $\frac{12692293\zeta(3)}{354294}-\frac{21248\zeta(3)^2}{2187}+\frac{110023\zeta(5)}{6561}+\frac{10976\zeta(7)}{243}+\frac{7012401169}{8503056}+\frac{9319\pi^4}{65610}-\frac{40\pi^6}{15309}$ |
| | $n^{-6}$ | $\frac{70030813\zeta(3)}{177147}-\frac{2776\zeta(3)^2}{2187}-\frac{1317440\zeta(5)}{19683}-\frac{9310\zeta(7)}{243}-\frac{29401282657}{12754584}-\frac{2378\pi^4}{10935}+\frac{40\pi^6}{15309}$ |
| | $n^{-7}$ | $-\frac{49663720\zeta(3)}{59049}+\frac{12544\zeta(3)^2}{729}+\frac{248920\zeta(5)}{2187}+\frac{2156\zeta(7)}{243}+\frac{5910065444}{1594323}+\frac{2968\pi^4}{32805}$ |
| | $n^{-8}$ | $\frac{120215648\zeta(3)}{177147}-\frac{21952\zeta(3)^2}{2187}-\frac{118720\zeta(5)}{2187}-\frac{1839682880}{531441}$ |
| | $n^{-9}$ | $\frac{8360078384}{4782969}-\frac{35236096\zeta(3)}{177147}$ |
| | $n^{-10}$ | $-\frac{1767467744}{4782969}$ |

Table 10: Coefficients of $\varepsilon$ expansion for $\nu^{-1}$

| **Coef.** | | **Value** |
|---|---|---|
| $C^{(0)}_{\nu^{-1}}$ | | |
| | $n^0$ | $2$ |
| $C^{(1)}_{\nu^{-1}}$ | | |
| | $n^0$ | $-\frac{2}{3}$ |
| | $n^{-1}$ | $\frac{2}{3}$ |
| $C^{(2)}_{\nu^{-1}}$ | | |
| | $n^0$ | $\frac{19}{162}$ |
| | $n^{-1}$ | $-\frac{115}{54}$ |
| | $n^{-2}$ | $\frac{125}{27}$ |
| | $n^{-3}$ | $-\frac{212}{81}$ |
| $C^{(3)}_{\nu^{-1}}$ | | |
| | $n^0$ | $\frac{937}{17496}-\frac{4\zeta(3)}{27}$ |
| | $n^{-1}$ | $\frac{40\zeta(3)}{27}+\frac{27421}{17496}$ |
| | $n^{-2}$ | $-\frac{4\zeta(3)}{27}-\frac{146647}{8748}$ |
| | $n^{-3}$ | $\frac{104833}{2187}-\frac{16\zeta(3)}{3}$ |
| | $n^{-4}$ | $\frac{112\zeta(3)}{27}-\frac{116660}{2187}$ |
| | $n^{-5}$ | $\frac{44944}{2187}$ |
| $C^{(4)}_{\nu^{-1}}$ | | |
| | $n^0$ | $-\frac{119\zeta(3)}{1458}+\frac{40\zeta(5)}{81}+\frac{24857}{1889568}-\frac{\pi^4}{810}$ |
| | $n^{-1}$ | $-\frac{445\zeta(3)}{162}-\frac{40\zeta(5)}{9}+\frac{743923}{1889568}+\frac{\pi^4}{81}$ |
| | $n^{-2}$ | $\frac{11030\zeta(3)}{729}+\frac{160\zeta(5)}{81}+\frac{2660387}{157464}-\frac{\pi^4}{810}$ |
| | $n^{-3}$ | $\frac{220\zeta(3)}{27}+\frac{80\zeta(5)}{81}-\frac{39702473}{236196}-\frac{2\pi^4}{45}$ |
| | $n^{-4}$ | $-\frac{30308\zeta(3)}{243}+\frac{1520\zeta(5)}{81}+\frac{135376871}{236196}+\frac{14\pi^4}{405}$ |
| | $n^{-5}$ | $\frac{135376\zeta(3)}{729}-\frac{160\zeta(5)}{9}-\frac{17930803}{19683}$ |
| | $n^{-6}$ | $\frac{40762300}{59049}-\frac{59360\zeta(3)}{729}$ |
| | $n^{-7}$ | $-\frac{11910160}{59049}$ |
| $C^{(5)}_{\nu^{-1}}$ | | |
| | $n^0$ | $-\frac{3335\zeta(3)}{52488}+\frac{8\zeta(3)^2}{81}+\frac{176\zeta(5)}{729}-\frac{49\zeta(7)}{27}+\frac{64327}{204073344}-\frac{119\pi^4}{174960}+\frac{10\pi^6}{15309}$ |
| | $n^{-1}$ | $-\frac{5381\zeta(3)}{52488}+\frac{32\zeta(3)^2}{81}+\frac{19600\zeta(5)}{2187}+\frac{49\zeta(7)}{3}-\frac{7605311}{22674816}-\frac{89\pi^4}{3888}-\frac{10\pi^6}{1701}$ |
| | $n^{-2}$ | $-\frac{429469\zeta(3)}{13122}-\frac{224\zeta(3)^2}{81}-\frac{35669\zeta(5)}{729}-\frac{833\zeta(7)}{27}+\frac{370045}{354294}+\frac{1103\pi^4}{8748}+\frac{40\pi^6}{15309}$ |
| | $n^{-3}$ | $\frac{1023083\zeta(3)}{6561}-\frac{1120\zeta(3)^2}{81}+\frac{84203\zeta(5)}{2187}+\frac{3626\zeta(7)}{27}+\frac{1707416029}{8503056}+\frac{11\pi^4}{162}+\frac{20\pi^6}{15309}$ |
| | $n^{-4}$ | $\frac{1458977\zeta(3)}{6561}+\frac{3160\zeta(3)^2}{81}-\frac{50644\zeta(5)}{2187}-\frac{9653\zeta(7)}{27}-\frac{5438457853}{2834352}-\frac{7577\pi^4}{7290}+\frac{380\pi^6}{15309}$ |
| | $n^{-5}$ | $-\frac{15640772\zeta(3)}{6561}+\frac{2848\zeta(3)^2}{81}+\frac{316960\zeta(5)}{729}+\frac{8624\zeta(7)}{27}+\frac{5245252505}{708588}+\frac{16922\pi^4}{10935}-\frac{40\pi^6}{1701}$ |

Continued on next page

Table 10 Coefficients of $\varepsilon$ expansion for $\nu^{-1}$

| Coef. | | Value |
|---|---|---|
| | $n^{-6}$ | $\frac{32573192\zeta(3)}{6561}-\frac{10976\zeta(3)^2}{81}-\frac{1813400\zeta(5)}{2187}-\frac{2156\zeta(7)}{27}-\frac{7890324112}{531441}-\frac{1484\pi^4}{2187}$ |
| | $n^{-7}$ | $-\frac{28007680\zeta(3)}{6561}+\frac{6272\zeta(3)^2}{81}+\frac{33920\zeta(5)}{81}+\frac{2899226528}{177147}$ |
| | $n^{-8}$ | $\frac{8809024\zeta(3)}{6561}-\frac{1668995440}{177147}$ |
| | $n^{-9}$ | $\frac{3534935488}{1594323}$ |
| $C^{(6)}_{\nu^{-1}}$ | | |
| | $n^{0}$ | $\frac{244\zeta(3,5)}{243}+\frac{2\pi^4\zeta(3)}{1215}-\frac{68143\zeta(3)}{1889568}-\frac{16337\pi^8}{27556200}+\frac{29\pi^6}{78732}-\frac{667\pi^4}{1259712}-\frac{10365955}{7346640384}$ $+\frac{2519\zeta(3)^2}{6561}+\frac{256\zeta(3)^3}{729}+\frac{48077\zeta(5)}{472392}+\frac{736\zeta(3)\zeta(5)}{729}-\frac{2491\zeta(7)}{2916}+\frac{46112\zeta(9)}{6561}$ |
| | $n^{-1}$ | $-\frac{10916\zeta(3,5)}{1215}+\frac{8\pi^4\zeta(3)}{1215}+\frac{593441\zeta(3)}{629856}+\frac{733309\pi^8}{137781000}+\frac{9395\pi^6}{826686}-\frac{5381\pi^4}{6298560}-\frac{1838556691}{7346640384}$ $-\frac{962\zeta(3)^2}{729}-\frac{2368\zeta(3)^3}{729}-\frac{250573\zeta(5)}{472392}-\frac{12764\zeta(3)\zeta(5)}{729}-\frac{47377\zeta(7)}{1458}-\frac{435608\zeta(9)}{6561}$ |
| | $n^{-2}$ | $\frac{3364\zeta(3,5)}{135}-\frac{56\pi^4\zeta(3)}{1215}+\frac{5717177\zeta(3)}{1417176}-\frac{185021\pi^8}{15309000}-\frac{17821\pi^6}{275562}-\frac{429469\pi^4}{1574640}-\frac{22559133701}{3673320192}$ $+\frac{251075\zeta(3)^2}{13122}+\frac{6592\zeta(3)^3}{729}+\frac{3927689\zeta(5)}{39366}+\frac{45848\zeta(3)\zeta(5)}{729}+\frac{1560847\zeta(7)}{5832}+\frac{1238792\zeta(9)}{6561}$ |
| | $n^{-3}$ | $-\frac{123304\zeta(3,5)}{1215}-\frac{56\pi^4\zeta(3)}{243}-\frac{32404163\zeta(3)}{78732}+\frac{3501193\pi^8}{68890500}+\frac{87119\pi^6}{1653372}+\frac{1023083\pi^4}{787320}-\frac{106170937}{4782969}$ $-\frac{628277\zeta(3)^2}{13122}-\frac{22976\zeta(3)^3}{729}-\frac{2963083\zeta(5)}{6561}-\frac{78268\zeta(3)\zeta(5)}{729}-\frac{7822601\zeta(7)}{5832}-\frac{4335112\zeta(9)}{6561}$ |
| | $n^{-4}$ | $\frac{38468\zeta(3,5)}{243}+\frac{158\pi^4\zeta(3)}{243}+\frac{1225346087\zeta(3)}{708588}-\frac{2939989\pi^8}{27556200}-\frac{13228\pi^6}{413343}+\frac{1458977\pi^4}{787320}+\frac{97239977053}{38263752}$ $-\frac{2718784\zeta(3)^2}{6561}+\frac{25024\zeta(3)^3}{729}+\frac{7722835\zeta(5)}{39366}+\frac{9920\zeta(3)\zeta(5)}{729}+\frac{950417\zeta(7)}{162}+\frac{5320904\zeta(9)}{6561}$ |
| | $n^{-5}$ | $\frac{36544\zeta(3,5)}{405}+\frac{712\pi^4\zeta(3)}{1215}+\frac{776293441\zeta(3)}{177147}+\frac{207098\pi^8}{5740875}+\frac{11320\pi^6}{19683}-\frac{3910193\pi^4}{196830}-\frac{1816761374713}{76527504}$ $+\frac{890632\zeta(3)^2}{729}+\frac{16256\zeta(3)^3}{243}-\frac{114031\zeta(5)}{59049}+\frac{102400\zeta(3)\zeta(5)}{243}-\frac{3655529\zeta(7)}{243}+\frac{2232592\zeta(9)}{2187}$ |
| | $n^{-6}$ | $-\frac{387664\zeta(3,5)}{1215}-\frac{2744\pi^4\zeta(3)}{1215}-\frac{279035720\zeta(3)}{6561}+\frac{2301209\pi^8}{34445250}-\frac{453350\pi^6}{413343}+\frac{4071649\pi^4}{98415}+\frac{3843591284657}{38263752}$ $+\frac{7405228\zeta(3)^2}{6561}-\frac{97280\zeta(3)^3}{729}+\frac{444158720\zeta(5)}{59049}-\frac{904096\zeta(3)\zeta(5)}{729}+\frac{14031773\zeta(7)}{729}-\frac{15030784\zeta(9)}{6561}$ |
| | $n^{-7}$ | $\frac{188416\zeta(3,5)}{1215}+\frac{1568\pi^4\zeta(3)}{1215}+\frac{19525189904\zeta(3)}{177147}-\frac{683008\pi^8}{17222625}+\frac{8480\pi^6}{15309}-\frac{700192\pi^4}{19683}-\frac{2279709378751}{9565938}$ $-\frac{45209600\zeta(3)^2}{6561}+\frac{41984\zeta(3)^3}{729}-\frac{1275519016\zeta(5)}{59049}+\frac{1195904\zeta(3)\zeta(5)}{729}-\frac{8134784\zeta(7)}{729}+\frac{6497920\zeta(9)}{6561}$ |
| | $n^{-8}$ | $-\frac{24379661096\zeta(3)}{177147}+\frac{51317504\zeta(3)^2}{6561}+\frac{1293727120\zeta(5)}{59049}-\frac{62720\zeta(3)\zeta(5)}{81}+\frac{1599752\zeta(7)}{729}+\frac{1616890953748}{4782969}+\frac{1101128\pi^4}{98415}$ |
| | $n^{-9}$ | $\frac{5037622016\zeta(3)}{59049}-\frac{18615296\zeta(3)^2}{6561}-\frac{50337280\zeta(5)}{6561}-\frac{4095193082848}{14348907}$ |
| | $n^{-10}$ | $\frac{1902028731680}{14348907}-\frac{3735026176\zeta(3)}{177147}$ |
| | $n^{-11}$ | $-\frac{374703161728}{14348907}$ |

Table 11: Coefficients of $\varepsilon$ expansion for $\gamma$

| **Coef.** | | **Value** |
|---|---|---|
| $C_\gamma^{(0)}$ | | |
| | $n^0$ | $1$ |
| $C_\gamma^{(1)}$ | | |
| | $n^0$ | $\frac{1}{3}$ |
| | $n^{-1}$ | $-\frac{1}{3}$ |
| $C_\gamma^{(2)}$ | | |
| | $n^0$ | $\frac{7}{162}$ |
| | $n^{-1}$ | $\frac{5}{6}$ |
| | $n^{-2}$ | $-\frac{59}{27}$ |
| | $n^{-3}$ | $\frac{106}{81}$ |
| $C_\gamma^{(3)}$ | | |
| | $n^0$ | $\frac{2\zeta(3)}{27}-\frac{361}{8748}$ |
| | $n^{-1}$ | $-\frac{20\zeta(3)}{27}-\frac{1027}{8748}$ |
| | $n^{-2}$ | $\frac{2\zeta(3)}{27}+\frac{13301}{2187}$ |
| | $n^{-3}$ | $\frac{8\zeta(3)}{3}-\frac{46586}{2187}$ |
| | $n^{-4}$ | $\frac{56104}{2187}-\frac{56\zeta(3)}{27}$ |
| | $n^{-5}$ | $-\frac{22472}{2187}$ |
| $C_\gamma^{(4)}$ | | |
| | $n^0$ | $\frac{287\zeta(3)}{2916}-\frac{20\zeta(5)}{81}-\frac{17725}{472392}+\frac{\pi^4}{1620}$ |
| | $n^{-1}$ | $\frac{767\zeta(3)}{972}+\frac{20\zeta(5)}{9}-\frac{58403}{118098}-\frac{\pi^4}{162}$ |
| | $n^{-2}$ | $-\frac{4999\zeta(3)}{729}-\frac{80\zeta(5)}{81}-\frac{78121}{39366}+\frac{\pi^4}{1620}$ |
| | $n^{-3}$ | $-\frac{590\zeta(3)}{243}-\frac{40\zeta(5)}{81}+\frac{27226733}{472392}+\frac{\pi^4}{45}$ |
| | $n^{-4}$ | $\frac{14318\zeta(3)}{243}-\frac{760\zeta(5)}{81}-\frac{28562327}{118098}-\frac{7\pi^4}{405}$ |
| | $n^{-5}$ | $-\frac{66512\zeta(3)}{729}+\frac{80\zeta(5)}{9}+\frac{16575067}{39366}$ |
| | $n^{-6}$ | $\frac{29680\zeta(3)}{729}-\frac{19791260}{59049}$ |
| | $n^{-7}$ | $\frac{5955080}{59049}$ |
| $C_\gamma^{(5)}$ | | |
| | $n^0$ | $\frac{4537\zeta(3)}{52488}-\frac{4\zeta(3)^2}{81}-\frac{76\zeta(5)}{243}+\frac{49\zeta(7)}{54}-\frac{814133}{51018336}+\frac{287\pi^4}{349920}-\frac{5\pi^6}{15309}$ |
| | $n^{-1}$ | $\frac{48871\zeta(3)}{52488}-\frac{16\zeta(3)^2}{81}-\frac{5840\zeta(5)}{2187}-\frac{49\zeta(7)}{6}-\frac{325771}{2125764}+\frac{767\pi^4}{116640}+\frac{5\pi^6}{1701}$ |
| | $n^{-2}$ | $\frac{53695\zeta(3)}{6561}+\frac{112\zeta(3)^2}{81}+\frac{10543\zeta(5)}{486}+\frac{833\zeta(7)}{54}-\frac{80139941}{17006112}-\frac{4999\pi^4}{87480}-\frac{20\pi^6}{15309}$ |
| | $n^{-3}$ | $-\frac{449785\zeta(3)}{6561}+\frac{560\zeta(3)^2}{81}-\frac{80723\zeta(5)}{4374}-\frac{1813\zeta(7)}{27}-\frac{10064443}{354294}-\frac{59\pi^4}{2916}-\frac{10\pi^6}{15309}$ |
| | $n^{-4}$ | $-\frac{440656\zeta(3)}{6561}-\frac{1580\zeta(3)^2}{81}+\frac{12422\zeta(5)}{2187}+\frac{9653\zeta(7)}{54}+\frac{2676780037}{4251528}+\frac{7159\pi^4}{14580}-\frac{190\pi^6}{15309}$ |
| | $n^{-5}$ | $\frac{6993334\zeta(3)}{6561}-\frac{1424\zeta(3)^2}{81}-\frac{148880\zeta(5)}{729}-\frac{4312\zeta(7)}{27}-\frac{1588627858}{531441}-\frac{8314\pi^4}{10935}+\frac{20\pi^6}{1701}$ |
| Continued on next page | | |

Table 11 Coefficients of $\varepsilon$ expansion for $\gamma$

| Coef. | | Value |
|---|---|---|
| | $n^{-6}$ | $-\frac{15513280\zeta(3)}{6561}+\frac{5488\zeta(3)^2}{81}+\frac{891580\zeta(5)}{2187}+\frac{1078\zeta(7)}{27}+\frac{3515106391}{531441}+\frac{742\pi^4}{2187}$ |
| | $n^{-7}$ | $\frac{13754528\zeta(3)}{6561}-\frac{3136\zeta(3)^2}{81}-\frac{16960\zeta(5)}{81}-\frac{4099362538}{531441}$ |
| | $n^{-8}$ | $\frac{2445133376}{531441}-\frac{4404512\zeta(3)}{6561}$ |
| | $n^{-9}$ | $-\frac{1767467744}{1594323}$ |
| $C_\gamma^{(6)}$ | | |
| | $n^{0}$ | $-\frac{122\zeta(3,5)}{243}-\frac{\pi^4\zeta(3)}{1215}+\frac{9989\zeta(3)}{177147}+\frac{16337\pi^8}{55112400}-\frac{23\pi^6}{52488}+\frac{4537\pi^4}{6298560}-\frac{2152301}{918330048}$ $-\frac{2993\zeta(3)^2}{13122}-\frac{128\zeta(3)^3}{729}-\frac{208451\zeta(5)}{944784}-\frac{368\zeta(3)\zeta(5)}{729}+\frac{6607\zeta(7)}{5832}-\frac{23056\zeta(9)}{6561}$ |
| | $n^{-1}$ | $\frac{5458\zeta(3,5)}{1215}-\frac{4\pi^4\zeta(3)}{1215}-\frac{3235\zeta(3)}{118098}-\frac{733309\pi^8}{275562000}-\frac{5435\pi^6}{1653372}+\frac{48871\pi^4}{6298560}+\frac{276076031}{1836660096}$ $+\frac{947\zeta(3)^2}{2187}+\frac{1184\zeta(3)^3}{729}-\frac{2532365\zeta(5)}{944784}+\frac{6382\zeta(3)\zeta(5)}{729}+\frac{27679\zeta(7)}{2916}+\frac{217804\zeta(9)}{6561}$ |
| | $n^{-2}$ | $-\frac{1682\zeta(3,5)}{135}+\frac{28\pi^4\zeta(3)}{1215}+\frac{9945103\zeta(3)}{944784}+\frac{185021\pi^8}{30618000}+\frac{5267\pi^6}{183708}+\frac{10739\pi^4}{157464}-\frac{971147}{14348907}$ $-\frac{198695\zeta(3)^2}{26244}-\frac{3296\zeta(3)^3}{729}-\frac{1838465\zeta(5)}{78732}-\frac{22924\zeta(3)\zeta(5)}{729}-\frac{1344463\zeta(7)}{11664}-\frac{619396\zeta(9)}{6561}$ |
| | $n^{-3}$ | $\frac{61652\zeta(3,5)}{1215}+\frac{28\pi^4\zeta(3)}{243}+\frac{287404501\zeta(3)}{2834352}-\frac{3501193\pi^8}{137781000}-\frac{83639\pi^6}{3306744}-\frac{89957\pi^4}{157464}-\frac{28719398807}{612220032}$ $+\frac{707681\zeta(3)^2}{26244}+\frac{11488\zeta(3)^3}{729}+\frac{4540981\zeta(5)}{26244}+\frac{39134\zeta(3)\zeta(5)}{729}+\frac{7131113\zeta(7)}{11664}+\frac{2167556\zeta(9)}{6561}$ |
| | $n^{-4}$ | $-\frac{19234\zeta(3,5)}{243}-\frac{79\pi^4\zeta(3)}{243}-\frac{1080045767\zeta(3)}{1417176}+\frac{2939989\pi^8}{55112400}+\frac{3389\pi^6}{413343}-\frac{55082\pi^4}{98415}-\frac{60771509963}{153055008}$ $+\frac{1207295\zeta(3)^2}{6561}-\frac{12512\zeta(3)^3}{729}-\frac{741287\zeta(5)}{13122}-\frac{4960\zeta(3)\zeta(5)}{729}-\frac{2682299\zeta(7)}{972}-\frac{2660452\zeta(9)}{6561}$ |
| | $n^{-5}$ | $-\frac{18272\zeta(3,5)}{405}-\frac{356\pi^4\zeta(3)}{1215}-\frac{101441989\zeta(3)}{78732}-\frac{103549\pi^8}{5740875}-\frac{37220\pi^6}{137781}+\frac{3496667\pi^4}{393660}+\frac{1150805513827}{153055008}$ $-\frac{1314932\zeta(3)^2}{2187}-\frac{8128\zeta(3)^3}{243}-\frac{10157674\zeta(5)}{59049}-\frac{51200\zeta(3)\zeta(5)}{243}+\frac{1178297\zeta(7)}{162}-\frac{1116296\zeta(9)}{2187}$ |
| | $n^{-6}$ | $\frac{193832\zeta(3,5)}{1215}+\frac{1372\pi^4\zeta(3)}{1215}+\frac{6416583263\zeta(3)}{354294}-\frac{2301209\pi^8}{68890500}+\frac{222895\pi^6}{413343}-\frac{387832\pi^4}{19683}-\frac{747325462223}{19131876}$ $-\frac{3280562\zeta(3)^2}{6561}+\frac{48640\zeta(3)^3}{729}-\frac{192206800\zeta(5)}{59049}+\frac{452048\zeta(3)\zeta(5)}{729}-\frac{13809803\zeta(7)}{1458}+\frac{7515392\zeta(9)}{6561}$ |
| | $n^{-7}$ | $-\frac{94208\zeta(3,5)}{1215}-\frac{784\pi^4\zeta(3)}{1215}-\frac{8995833160\zeta(3)}{177147}+\frac{341504\pi^8}{17222625}-\frac{4240\pi^6}{15309}+\frac{1719316\pi^4}{98415}+\frac{1964591142751}{19131876}$ $+\frac{22010080\zeta(3)^2}{6561}-\frac{20992\zeta(3)^3}{729}+\frac{606159968\zeta(5)}{59049}-\frac{597952\zeta(3)\zeta(5)}{729}+\frac{4044754\zeta(7)}{729}-\frac{3248960\zeta(9)}{6561}$ |
| | $n^{-8}$ | $\frac{3898850900\zeta(3)}{59049}-\frac{25428256\zeta(3)^2}{6561}-\frac{635644520\zeta(5)}{59049}+\frac{31360\zeta(3)\zeta(5)}{81}-\frac{799876\zeta(7)}{729}-\frac{740758735136}{4782969}-\frac{550564\pi^4}{98415}$ |
| | $n^{-9}$ | $-\frac{7433106688\zeta(3)}{177147}+\frac{9307648\zeta(3)^2}{6561}+\frac{25168640\zeta(5)}{6561}+\frac{1952912589656}{14348907}$ |
| | $n^{-10}$ | $\frac{1867513088\zeta(3)}{177147}-\frac{932455954528}{14348907}$ |
| | $n^{-11}$ | $\frac{187351580864}{14348907}$ |
